# Supplementary material for: Identifying and Mapping Cell-type Specific Chromatin Programming of Gene Expression
Source: arXiv:1210.3313 source file (2012-10-11)
Supplement: Supplementary file 1 [file arxiv_SI.pdf]

# SUPPLEMENTARY INFORMATION: Identifying and Mapping Cell-type Specific Chromatin Programming of Gene Expression

Troels T. Marstrand[1] and John D. Storey[1,2*]

[1]Lewis-Sigler Institute for Integrative Genomics
[2]Department of Molecular Biology
Princeton University, Princeton, NJ 08544, USA.
*Corresponding author: jstorey@princeton.edu

# Supplementary Material

**ARS versus standard correlation measures.** While the standard Pearson correlation statistic is capable of capturing some instances of cell-type specific outliers that are also detected by our proposed ARS method, the operating characteristics of the correlation statistic are unreliable when the data are not Normal and there are outliers. In comparing a test of non-zero correlation to our method, we predicted a total of 1566 significant genes using the parametric correlation test (`cor.test` in R) compared to 2538 with our proposed method at FDR $< 0.05$. However, upon further investigation it became clear that the correlation test identifies cases that are not of biological interest and it has unreliable behavior due to outliers (which are of biological interest). Furthermore, the data are not Normal distributed, which means that the p-values produced by the function `cor.test` are not trustworthy.

To illustrate the point that the Pearson statistic identifies cases that are not of biological interest, Figure S2 shows instances where the Pearson correlation statistic and the ARS statistic either agree or differ. The top left panel shows an example where both $\text{ARS}_{\text{max}}$ and correlation produce significant p-values. The bottom left shows an example where correlation produces a biological false positive. The top and bottom right are more or less indistinguishable, but the correlation test gives widely different results while our ARS remains stable and rightfully calls both genes as having a distinct outlier.

Furthermore the parametric p-values generated from the standard Pearson correlation test are not valid when data for a given gene are not bivariate Normal, as is the case with the data considered here. We investigated the Normal assumption by testing the data, DHS and gene expression for each gene, against the Normal by using a Kolomogorov-Smirnov test. The $\sim$21,000 resulting p-values were then further tested against Uniform(0,1), which identifies if there are systematic departures from Normality. We would expect the p-values to be Uniform had the tests against Normal been non-significant across all genes. The p-values from this nested Kolomogorov-Smirnov procedure proved data to be not Normal, with p-value $<$ 2.2e-16 in all cases (Figure S3 shows the results for DHS segment size $\pm$ 2.5kb, and DHS segment size $\pm$ 200kb).

Instead of using parametric p-values from the Pearson correlations, we investigated the performance of the Pearson correlation using our randomization strategy. We assigned p-values to the obtained correlations from the observed data, based on correlations obtained using randomized data exactly as it was generated for the ARS method (100 total iterations, same as the ARS method). This resulted in the estimated proportion of true null genes to be $\hat{\pi}_0 = 1$, implying that there is no biological signal since no test was significant when correcting for multiple testing (Figure S4). This is in contrast to the statistic reported in the main text that the ARS method estimates that about 25% of the genes show the signal of interest. Finally, log-transforming the data in order to better approximate the Normal does not alleviate the problem and Pearson correlations still resulted in $\hat{\pi}_0 = 1$.

We further tested the performance of the rank-based Spearman correlation test, as this would indicate a simple monotonic trend between the variables, gene expression and DHS. However, the power of the Spearman correlation over an order of magnitude less than the ARS statistic, as can be seen in Figure S5, and S6.

**Aggregation test.** To test for an aggregation of significant genes from the same cell-type in terms of genomic location, we counted the number of cell-type matching significant genes within a boundary of 100kb. We tested against two different null models: (i) pairs of random significant genes (no boundary) or (ii) the fraction of neighboring genes with an outlier in matching cell-types, irrespective of significance. Both null models confirmed the presence of aggregation and possible regulatory islands at extreme significance (Fishers exact test p-values $<$ 2.2e-16). We also tested aggregation by considering the number of genes as well as the distance between significant gene pairs from the same cell-type versus that of non-significant genes pairs. Using both measurements we find that significant ARS genes tend to aggregate (Kolmogorov-Smirnov test p-values $<$ 2.2e-16 for both, Figure S15).

**Experimental replication.** Assessment of reproducibility was done by pairing DHS volume and gene expression of two replicates from 10 cell-types, such that we got a total of four pairings A1, B1, A2, and B2, with A, B representing DHS replicates and 1, 2 representing gene expression replicates. Next we calculated the fraction of significant genes (FDR $<$ 0.05) from one pairing retained in another, and did this for all four-way comparisons (Figure S16).

**Determining the angular penalty rate $c$.** Recall from the main text that for a given segment size and gene, the DHS volume data and gene expression data are scaled and medoid centered, represented by $m$-vectors $\mathbf{x}^*$ and $\mathbf{y}^*$, respectively (here, $m = 20$ cell lines). We calculate $d_i = \sqrt{x_i^{*2} + y_i^{*2}}$ for $i = 1, 2, \ldots, m$ to obtain the "ratio" component of the angle-ratio statistic (ARS) calculated as $r_i = \frac{d_i}{\text{med}(\mathbf{d})}$. We then calculate the angle $\theta_i$ for each data point $(x_i^*, y_i^*)$ relative to the unit vector $(1, 0)$, where $0 \leq \theta_i \leq 360$. The angular penalty involves first calculating the smaller of the two angular distances between $\theta_i$ and the identity line, calculated by:

$$\Delta_i = \begin{cases} |45 - \theta_i| & \text{for } 0 \leq \theta_i < 135 \\ |225 - \theta_i| & \text{for } 135 \leq \theta_i < 315 \\ |45 - (\theta_i - 360)| & \text{for } 315 \leq \theta_i < 360 \end{cases}$$

The angular penalty is calculated as $a_i = \exp(c \times \Delta_i)$. ARS is then based on the product $\text{ARS}_i = a_i \times r_i$ as described in the text. The correct value of $c$ is that which captures the distribution of angles among true null genes. The most direct way to determine this value is to identify the value of $c$ such that the genes ranked least significant according to ARS produce valid null p-values. This can be accomplished by performing a statistical test of whether the large p-values follow the Uniform distribution. As can be seen from the p-value histograms in Figure S12, incorrect values of $c$ lead to either conservative or anti-conservative p-value estimates in the right tail. Within a narrow range of $c$ values, the null p-values were Uniform according to a Kolmogorov-Smirnov test, and this range was similar across all segments of DHS volume tested (Figure S12).

**Null data randomization strategy.** In resampling the data to obtain a correct null ARS distribution, the dependence between expression and DHS volume is retained by treating each

2-tuple as the unit to resample $(x_i, y_i)$ as well as the angle $\theta_i$ associated with 2-tuple. In order to make the data exchangeable across genes, we actually resample the scaled data $(x_i^s, y_i^s)$, as defined in the main text. Finally, as "outliers" are not uniformly distributed across the cell-types under consideration, our permutation strategy should be balanced across cell-types. The data for a given gene can take one of two possible configurations:

$$\text{Case 1}: \begin{bmatrix} x_1^s < 1 & y_1^s < 1 \\ \vdots & \vdots \\ x_i^s = 1 & y_i^s = 1 \\ \vdots & \vdots \\ x_m^s < 1 & y_m^s < 1 \end{bmatrix}, \ \text{Case 2}: \begin{bmatrix} x_1^s < 1 & y_1^s < 1 \\ \vdots & \vdots \\ x_i^s = 1 & y_i^s < 1 \\ \vdots & \vdots \\ x_j^s < 1 & y_j^s = 1 \\ \vdots & \vdots \\ x_m^s < 1 & y_m^s < 1 \end{bmatrix}$$

This can be understood in terms of Figure S9, which is a plot of the scaled data. Case 1 is a gene such that one of the cell line's 2-tuple lies on the upper right corner, point $(1, 1)$, and all other $m-1$ points lie in the interior of the unit square. Case 2 is a gene such that one cell line's 2-tuple lies on the top boundary $(x, 1)$, another cell line's 2-tuple lies on the right boundary $(1, y)$, and the other $m-2$ points lie in the interior of the unit square. This phenomenon is simply due to the way in which the data are scaled. We take it into account, however, when generating randomized data.

The strategy we take to generate a "null" gene's data is to randomly sample $m$ points from Figure S9, but do so in a way that the cell lines are balanced and the two cases are represented proportionally. Moreover, when we randomly sample a point, we take with it the observed angle and utilize that angle in the ARS calculation for the null gene. The following provides the details of the algorithm.

We extend the notation by writing 2-tuples as $(x_{ij}^s, y_{ij}^s)$ where $i$ denotes the cell line as before and $j$ denotes the gene ($i = 1, \ldots, m$; $j = 1, \ldots, N$). Here, $m = 20$ and $N = 19,215$. This allows us to classify all such 2-tuples into $m + 3$ different sets:

$$\begin{aligned} \mathcal{B}_{\text{corner}} &= \{(x_{ij}^s, y_{ij}^s) : (x_{ij}^s, y_{ij}^s) = (1,1)\} \\ \mathcal{B}_{\text{top}} &= \{(x_{ij}^s, y_{ij}^s) : x_{ij}^s < 1, y_{ij}^s = 1\} \\ \mathcal{B}_{\text{right}} &= \{(x_{ij}^s, y_{ij}^s) : x_{ij}^s = 1, y_{ij}^s < 1\} \\ \mathcal{C}_k &= \{(x_{ij}^s, y_{ij}^s) : i = k, x_{kj}^s < 1, y_{kj}^s < 1\}, \end{aligned}$$

where $\mathcal{C}_k$ is defined for $k = 1, 2, \ldots, m$. It can be seen that $\mathcal{B}_{\text{corner}}$ contains top right corner points, $\mathcal{B}_{\text{top}}$ contains the top boundary points, $\mathcal{B}_{\text{right}}$ contains the right boundary points, and the $\mathcal{C}_k$ contain the interior points for each respective cell line.

Let $r$ be the proportion of genes that fall into Case 1 and $1 - r$ the proportion that fall into Case 2. The algorithm to generate a randomized data set works as follows:

1. Assign a fraction $r$ of genes to Case 1 and $1 - r$ to Case 2.

2. For each gene of Case 1, randomly assign a 2-tuple from $\mathcal{B}_{\text{corner}}$, and record its cell line, $k_{\text{corner}}$. Randomly assign one 2-tuple from each $\mathcal{C}_k$ for all $k \neq k_{\text{corner}}$ to the gene. This yields a gene of exactly $m$ 2-tuples of type Case 1, with one 2-tuple from each cell line.

3. For each gene of Case 2, randomly assign a 2-tuple from $\mathcal{B}_{\text{top}}$, and record its cell line, $k_{\text{top}}$. Also randomly assign a 2-tuple from $\mathcal{B}_{\text{right}}$, and record its cell line, $k_{\text{right}}$. We do so such that $k_{\text{top}} \neq k_{\text{right}}$. Then randomly assign to the gene one 2-tuple from each $\mathcal{C}_k$ for all $\{k : k \neq k_{\text{top}} \text{ and } k \neq k_{\text{right}}\}$. This yields a gene of exactly $m$ 2-tuples of type Case 2, with one 2-tuple from each cell line.

Once the randomized genes are formed, the data for each gene are median centered, and then the ratio statistic is calculated. Recall that the angles are tied their original 2-tuples. Therefore, the angular penalty applied to each 2-tuple is exactly that from the original data set. From these $\text{ARS}_i$ statistics, the $\text{ARS}_{\text{max}}$ statistic is then calculated for each randomized gene.

This entire process is repeated for $B$ total permutation data sets to produce $B$ sets of $N$ randomized $\text{ARS}_{\text{max}}$ statistics. The proportion of these exceeding the observed $\text{ARS}_{\text{max}}$ statistics then forms the basis of the p-values. We performed this procedure for $B$=3, 10 and 100.We then compared the distribution of the null-statistics to verify that the procedure quickly converges for a low number of permutations. If the distributions of randomized ARS values is identical among the values of $B$, then the p-values generated from any number of permutations would likewise be stable. In all cases the distribution of null statistics were identical according to a Kolmogorov-Smirnov test, 3 versus 10: p-value 0.75, 3 versus 100: p-value 0.54, 10 versus 100: p-value 0.67. The difference in estimated $\pi_0$ between 3 and 100 permutations was ~0.01 (0.8221462 versus 0.8315243), with the lower $\pi_0$ estimate achieved at 100 permutations resulting in 9 more genes being detected at FDR<0.01, and 30 more genes at FDR<0.05. To ensure stable, and high resolution p-values all reported p-values in the paper are based on 100 permutations.

**Local ARS profiles.** For a given gene, the gene expression data $\mathbf{x} = (x_1, \ldots, x_m)^T$ are fixed. The larger DHS segment is broken into $L$ consecutive non-overlapping smaller regions, forming a matrix

$$\mathbf{A} = \begin{bmatrix} y_{1,1} & \cdots & y_{1,l} & \cdots & y_{1,L} \\ \vdots & \ldots & \vdots & \ldots & \vdots \\ y_{i,1} & \cdots & y_{i,l} & \cdots & y_{i,L} \\ \vdots & \ldots & \vdots & \ldots & \vdots \\ y_{m,1} & \cdots & y_{m,l} & \cdots & y_{m,L} \end{bmatrix}.$$

Now the standard ARS is calculated for each column vector of $\mathbf{A}$, $\mathbf{y_l} = (y_1, \ldots, y_m)^T$ against the gene expression vector $\mathbf{x}$. From these data, we can obtain a matrix of $\text{ARS}_{i,l}$ for $i = 1, \ldots, m$ and $l = 1, \ldots, L$.

However, since each $\mathbf{y}_l$ is scaled individually (to produce $\mathbf{y}_l^s$ in forming the $\text{ARS}_{i,l}$), the resolution is lost across regions. We therefore scale the resulting $\text{ARS}_{i,l}$ for a fixed $l$

by its maximal DHS value relative to the average maximal DHS value across all regions. Specifically, let $\max_l = \max(y_{1,l}, \ldots, y_{m,l})$. We form

$$\text{ARS}^*_{i,l} = \frac{\max_l}{\sum_{k=1}^{L} \max_k / L} \text{ARS}_{i,l}.$$

thereby obtaining a matrix of local ARS scores:

$$\text{ARS}_{\text{local}} = \begin{bmatrix} \text{ARS}^*_{1,1} & \ldots & \text{ARS}^*_{1,l} & \ldots & \text{ARS}^*_{1,L} \\ \vdots & \ldots & \vdots & \ldots & \vdots \\ \text{ARS}^*_{i,1} & \ldots & \text{ARS}^*_{i,l} & \ldots & \text{ARS}^*_{i,L} \\ \vdots & \ldots & \vdots & \ldots & \vdots \\ \text{ARS}^*_{m,1} & \ldots & \text{ARS}^*_{m,l} & \ldots & \text{ARS}^*_{m,L} \end{bmatrix}.$$

By selecting the proper row vector $(\text{ARS}^*_{i,1}, \ldots, \text{ARS}^*_{i,L})$ for cell type $i$ where significance was established on the larger DHS segment, we now have a local measure of which hypersensitive sites contributed the most to the detected association.

# Supplementary Figures and Tables

| Symbol | Description | Vendor |
|---|---|---|
| AG04450 | fetal lung fibroblast | Coriell AG04450 |
| BJ | skin fibroblast | ATCC CRL-2522 |
| CACO2 | colorectal adenocarcinoma | ATCC HTB-37 |
| GM06990 | lymphoblastoid (CEPH) | Coriell GM06990 |
| H7-hESC | Undifferentiated human embryonic stem cells | WiCell WA07 (H7) |
| HAEpiC | Human Amniotic Epithelial Cells | ScienCell 7100 |
| HCF | Human cardiac fibroblasts | ScienCell 6300 |
| HCPEpiC | Human choroid plexus epithelial cells | ScienCell 1310 |
| HL-60 | Human promyelocytic leukemia cells | ATCC CCL-240 |
| HeLa | cervical carcinoma | ATCC CCL-2.2 |
| HepG2 | liver carcinoma | ATCC HB-8065 |
| HMEC | Human mammary epithelial cells | Lonza CC-3150 |
| HRCEpiC | Human renal cortical epithelial cells | ScienCell #4110 |
| HUVEC | Human Umbillical Vein Endothelial Cell | Lonza CC-2517 |
| PANC-1 | pancreatic carcinoma | ATCC CRL-1469 |
| K562 | leukemia | ATCC CCL-243 |
| SAEC | Small airway epithelial cells | Lonza CC-2547 |
| SK-N-SH_RA | neuroblastoma cell line differentiated w. retinoic acid | ATCC HTB-11 |
| SKMC | Human skeletal muscle cells | Lonza CC-2561 |
| TH1 | primary human Th1 T cells | None |

Table S1: **Cell-lines and vendors.** The 20 cell lines and primary cells used in the study were procured from commercial or other sources as listed above. Further information on growth conditions and protocols are available via:
http://genome.ucsc.edu/cgi-bin/hgEncodeVocab?type=cellType

| **Internal id** | **Cell-type** | **Alt. name** | **subId** |
|---|---|---|---|
| DS12255 | AG04450 | AG04450 | subId=907 |
| DS10018 | BJ | BJ | subId=393 |
| DS8235 | CACO2 | Caco-2 | subId=288 |
| DS7748 | GM06990 | GM06990 | subId=46 |
| DS11909 | hESCT0 | H7-hESC | subId=917 |
| DS12663 | HAEpiC | HAEpiC | subId=918 |
| DS12491 | HCF | HCF | subId=921 |
| DS12447 | HCPEpiC | HCPEpiC | subId=922 |
| DS11733 | HL60 | HL-60 | subId=507 |
| DS8680 | HMEC | HMEC | subId=627 |
| DS10662 | HRCE | HRCEpiC | subId=399 |
| DS10060 | HUVEC | HUVEC | subId=297 |
| DS10011 | Hela | HeLa-S3 | subId=396 |
| DS7764 | HEPG2 | HepG2 | subId=48 |
| DS9764 | K562 | K562 | subId=106 |
| DS9873 | PANC1 | PANC-1 | subId=511 |
| DS10514 | SAEC | SAEC | subId=513 |
| DS11939 | SkMC | SKMC | subId=754 |
| DS8476 | SKNSH | SK-N-SH_RA | subId=737 |
| DS7840 | TH1 | Th1 | subId=49 |

Table S2: **DNase I hypersensitive data.** The track IDs for each cell-type are specified and can be accessed via:
http://hgdownload.cse.ucsc.edu/goldenPath/hg18/encodeDCC/wgEncodeUwDnaseSeq/

| **Cell-type** | **subId** |
|---|---|
| BJ | 295 |
| BJ | 393 |
| Caco-2 | 288 |
| Caco-2 | 394 |
| GM06990 | 46 |
| GM06990 | 110 |
| HRCEpiC | 398 |
| HRCEpiC | 399 |
| HRE | 400 |
| HRE | 401 |
| HeLa-S3 | 396 |
| HeLa-S3 | 397 |
| HepG2 | 48 |
| HepG2 | 111 |
| K562 | 106 |
| K562 | 106 |
| SAEC | 514 |
| SAEC | 513 |
| SK-N-SH_RA | 50 |
| SK-N-SH_RA | 737 |

Table S3: **DNase I hypersensitive data - replicated.** The track IDs for each cell-type of the replicated data is specified and can be accessed via:
http://hgdownload.cse.ucsc.edu/goldenPath/hg18/encodeDCC/wgEncodeUwDnaseSeq/
Please note that the same subId for K562 appears twice as in the original file list from UCSC.

| **GEO-accession** | **Cell-type** |
|---|---|
| GSM510534 | AG04450-DS12255 |
| GSM472924 | BJ-DS11522 |
| GSM472933 | Caco-2-DS11539 |
| GSM472903 | GM06990-DS7748 |
| GSM510581 | H7-hESC-DS11909 |
| GSM510516 | HAEpiC-DS12663 |
| GSM510545 | HCF-DS12491 |
| GSM510547 | HCPEpiC-DS12447 |
| GSM472942 | HL-60-DS11733 |
| GSM472934 | HMEC-DS8680 |
| GSM472920 | HRCE-DS10662 |
| GSM472935 | HUVEC-DS10060 |
| GSM472905 | HeLa-S3-DS7930 |
| GSM472906 | HepG2-DS7764 |
| GSM472926 | K562-DS11524 |
| GSM472938 | PANC-1-DS9873 |
| GSM472923 | SAEC-DS10518 |
| GSM472943 | SKMC-DS11939 |
| GSM472912 | SK-N-SH_RA-DS8476 |
| GSM472914 | Th1-DS7840 |

Table S4: **GEO-accession number.** GEO-accession numbers for the Affymetrix exon-array data.

| **GEO-accession** | **Cell-type** |
|---|---|
| GSM472924 | BJ-DS11522 |
| GSM472925 | BJ-DS11523 |
| GSM472900 | Caco-2-DS8235 |
| GSM472933 | Caco-2-DS11539 |
| GSM472903 | GM06990-DS7748 |
| GSM472904 | GM06990-DS7784 |
| GSM472920 | HRCE-DS10662 |
| GSM472921 | HRCE-DS10666 |
| GSM472918 | HRE-DS10631 |
| GSM472919 | HRE-DS10641 |
| GSM472905 | HeLa-S3-DS7930 |
| GSM472916 | HeLa-S3-DS8200 |
| GSM472906 | HepG2-DS7764 |
| GSM472907 | HepG2-DS7768 |
| GSM472926 | K562-DS11524 |
| GSM472927 | K562-DS11525 |
| GSM472922 | SAEC-DS10514 |
| GSM472923 | SAEC-DS10518 |
| GSM472912 | SK-N-SH_RA-DS8476 |
| GSM472913 | SK-N-SH_RA-DS8482 |

Table S5: **GEO-accession number.** GEO-accession numbers for the replicated Affymetrix exon-array data.

Figure S1 *(following page)*: **Overview of ARS method, applied to example gene *CD69*.** *Step 1.* For a given gene, DHS volume and gene expression are calculated for all 20 cell lines as described in the text. DHS volume and gene expression are respectively scaled to lie on the unit interval [0,1] and then median centered before considering their joint distribution. Each cell-type corresponds to a single point. *Step 2.* In order to form the "ratio" component of the ARS statistic, $r_i$, the distance from the origin to each point is calculated and then scaled by the median distance (left panel). The angular distance between each point and the identity line is calculated and evaluated in an exponential function to determine an angular penalty $a_i$ for each cell type (right panel). *Step 3.* The final angle-ratio statistic (ARS) is computed as the product of the normalized distances and the angular penalties, $\text{ARS}_i = a_i \times r_i$. The maximal statistic $\text{ARS}_{\text{max}}$ is calculated for each gene and the corresponding cell-type recorded, in this case the TH1 cell line. *Step 4.* A randomization method is performed to generate null data, upon which null $\text{ARS}_{\text{max}}$ are calculated. These are compared to the observed $\text{ARS}_{\text{max}}$ values to calculate the statistical significance of each gene.

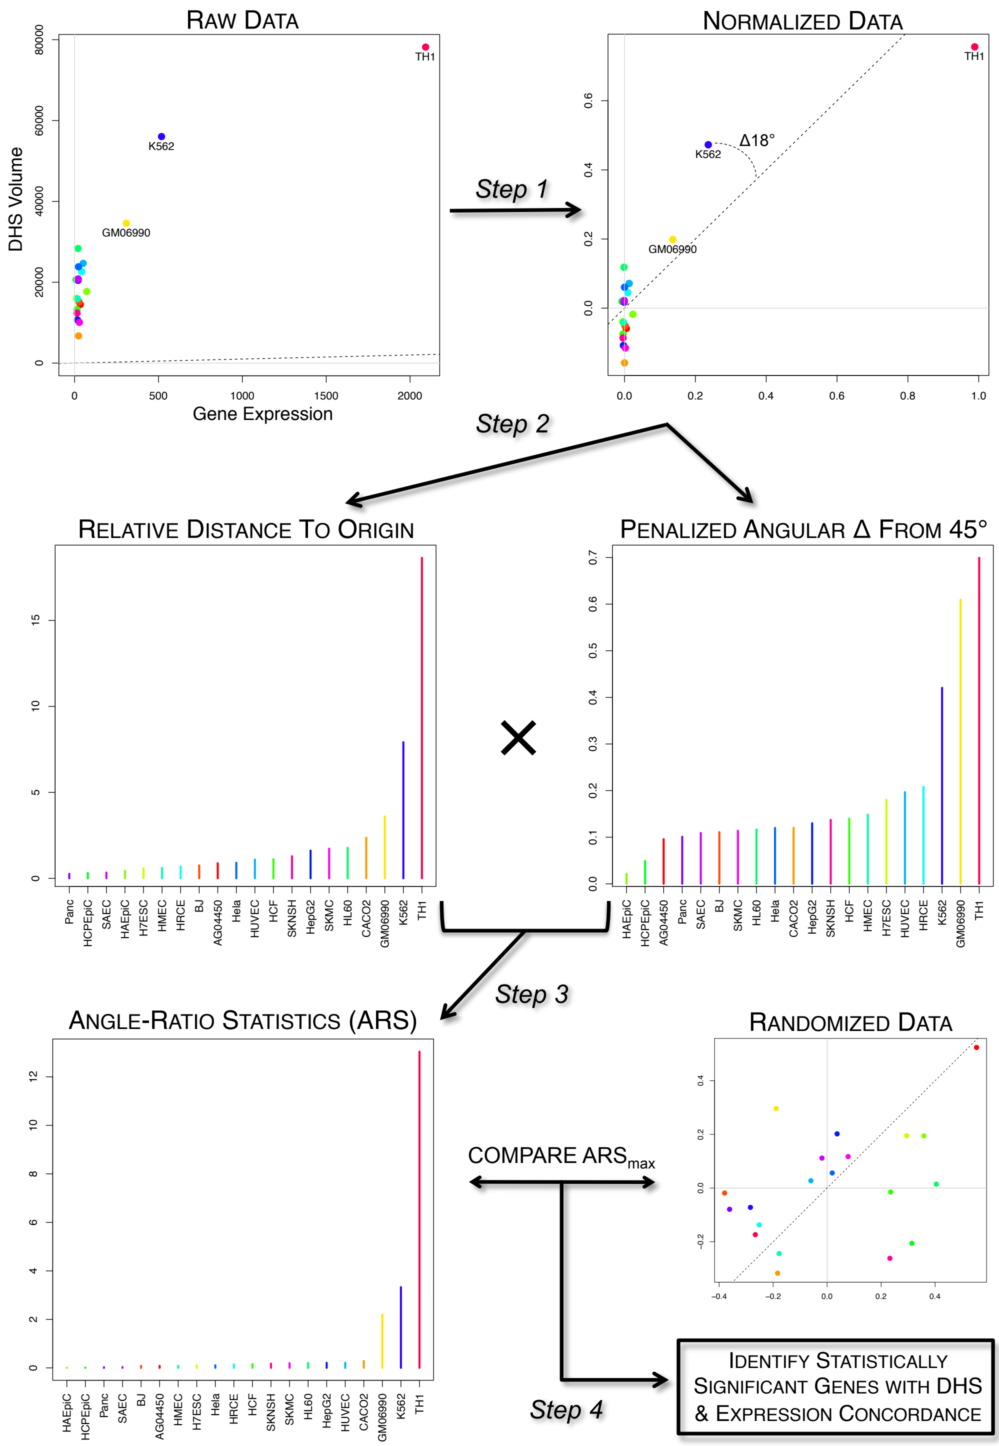
RAW DATA
DHS Volume
Gene Expression
TH1
K562
GM06990
Step 1
NORMALIZED DATA
Δ18°
Step 2
RELATIVE DISTANCE TO ORIGIN
PENALIZED ANGULAR Δ FROM 45°
×
Step 3
ANGLE-RATIO STATISTICS (ARS)
RANDOMIZED DATA
COMPARE ARSmax
Step 4
IDENTIFY STATISTICALLY SIGNIFICANT GENES WITH DHS & EXPRESSION CONCORDANCE

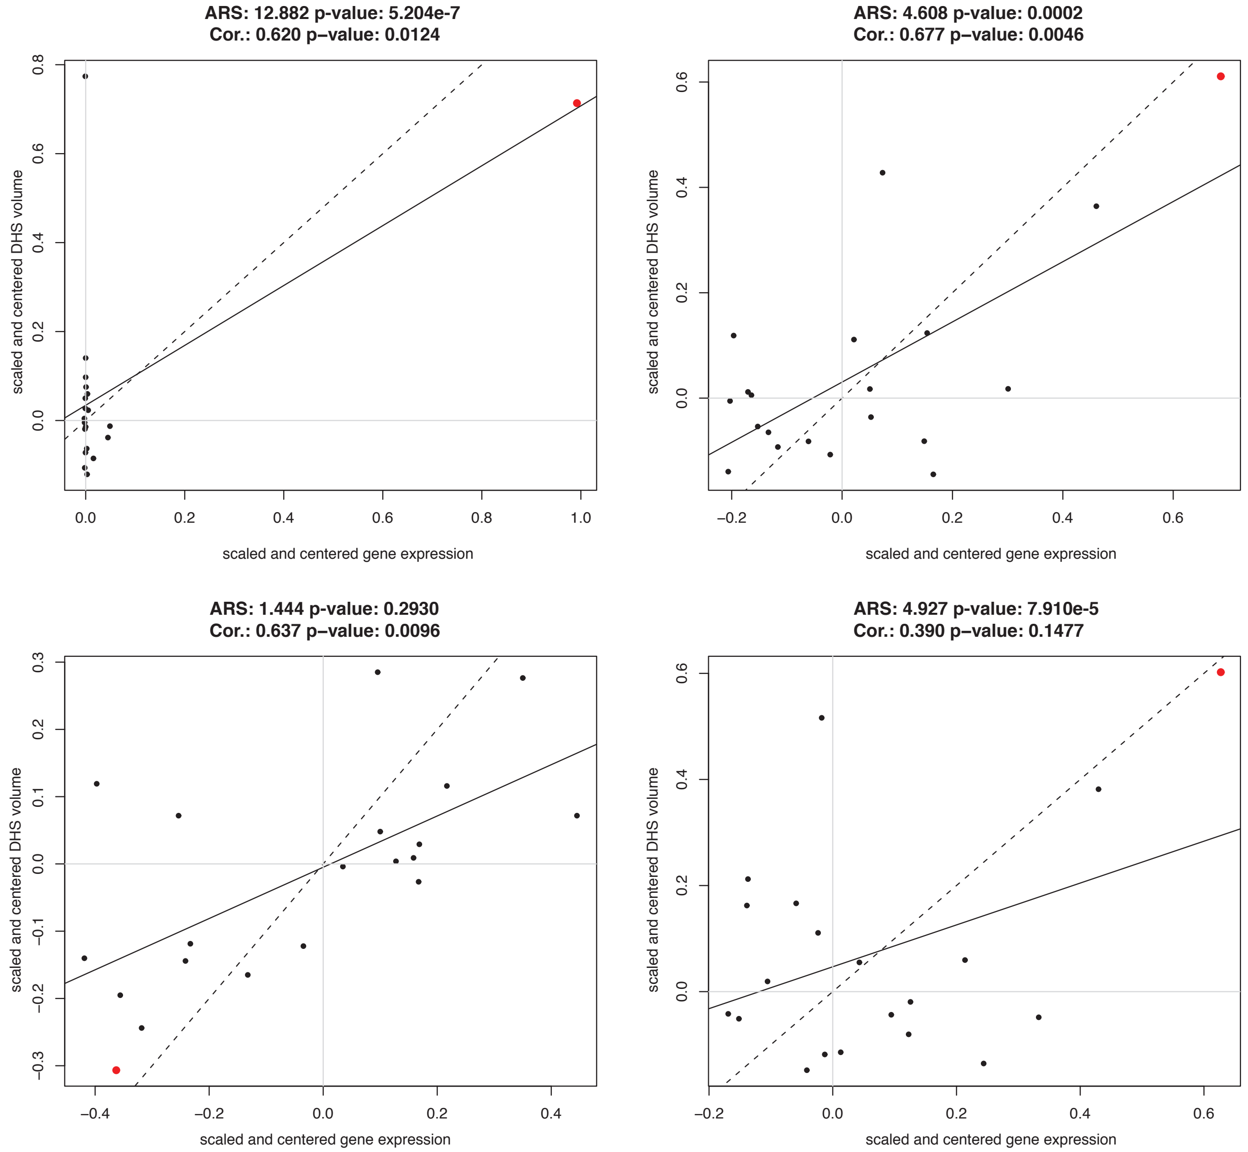


Figure S2: **Four examples of correlation versus angle ratio statistics (ARS).** Data points are represented by black dots and the outlier (i.e., most distant point to the origin) is the red point. The dashed line is the 45 degree identity line and the solid line is a standard regression line. The ARS and Pearson p-values are based on permuted data. To calculate ARS, the data, DHS and gene expression, were scaled by their maximum observations respectively and median centered. The distance and angle of the "outlier" relative to all other points determines the final test-statistic. ARS show robust detection of outliers while standard Pearson correlation may give spurious signals as data is not bivariate Normal. The genes under consideration are from the top right to bottom left *A2M, AADAT, ACSL3, ABCB6*

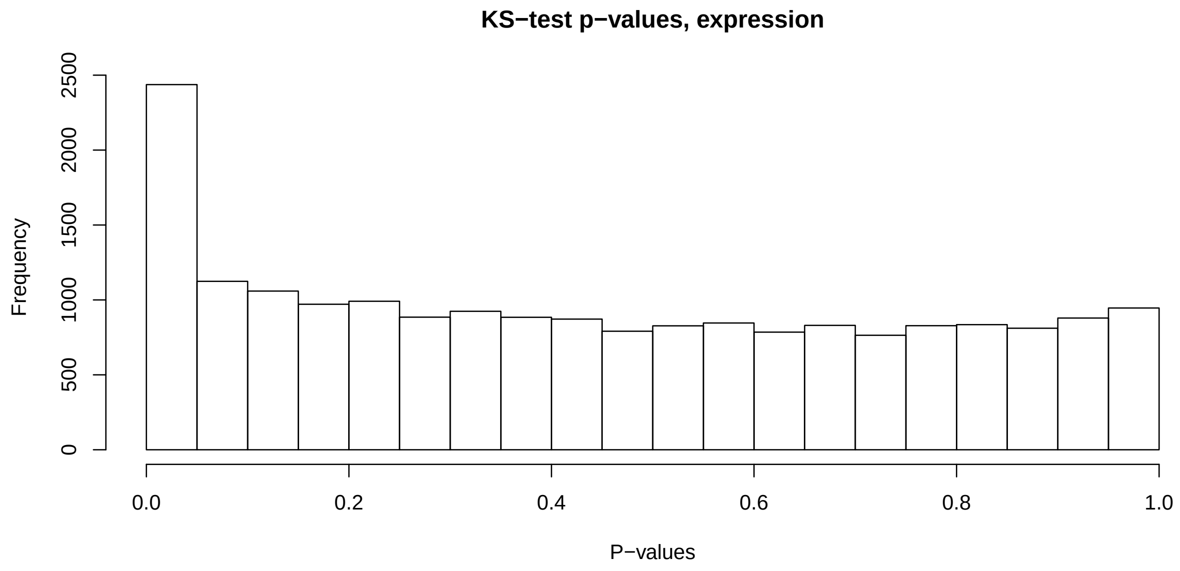


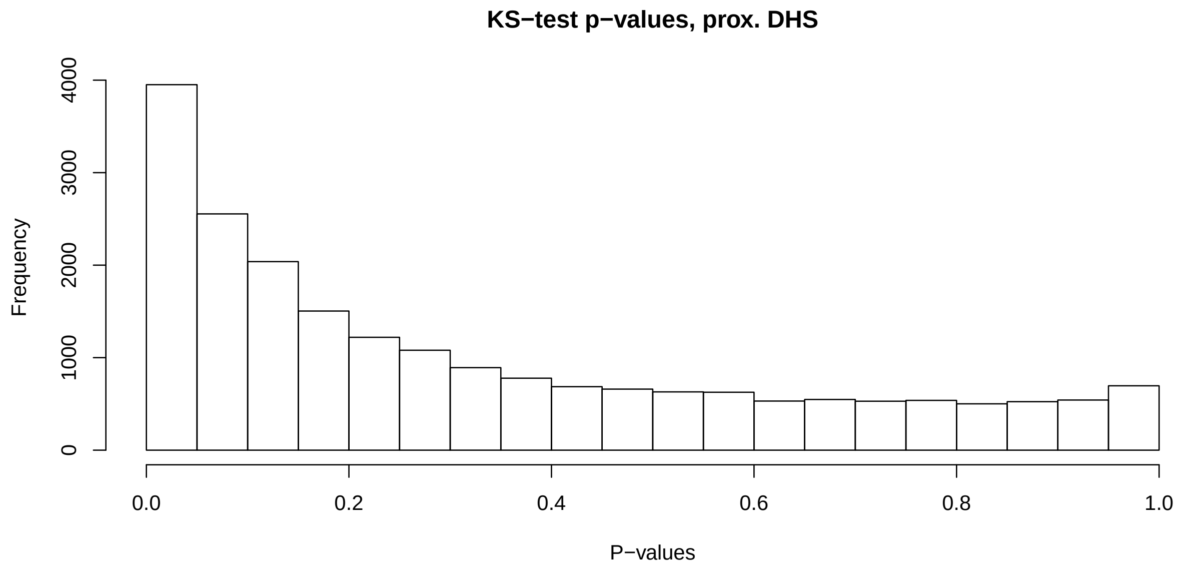


Figure S3: **Kolomogorov-Smirnov p-values testing whether gene expression and DHS data are Normal.** All expression data, and proximal ($\pm$ 2.5kb) DHS were centered and scaled on a per gene basis, and tested against Normal using a Kolmogorov-Smirnov test. The histograms show the distribution of the resulting p-values in both cases. If the data were Normal, a Uniform distribution would be present. In testing the resulting p-values against Uniform, using a Kolomogorov-Smirnov test we obtain p-values $<$ 2.2e-16 for both cases demonstrating that data cannot be assumed to be Normal.

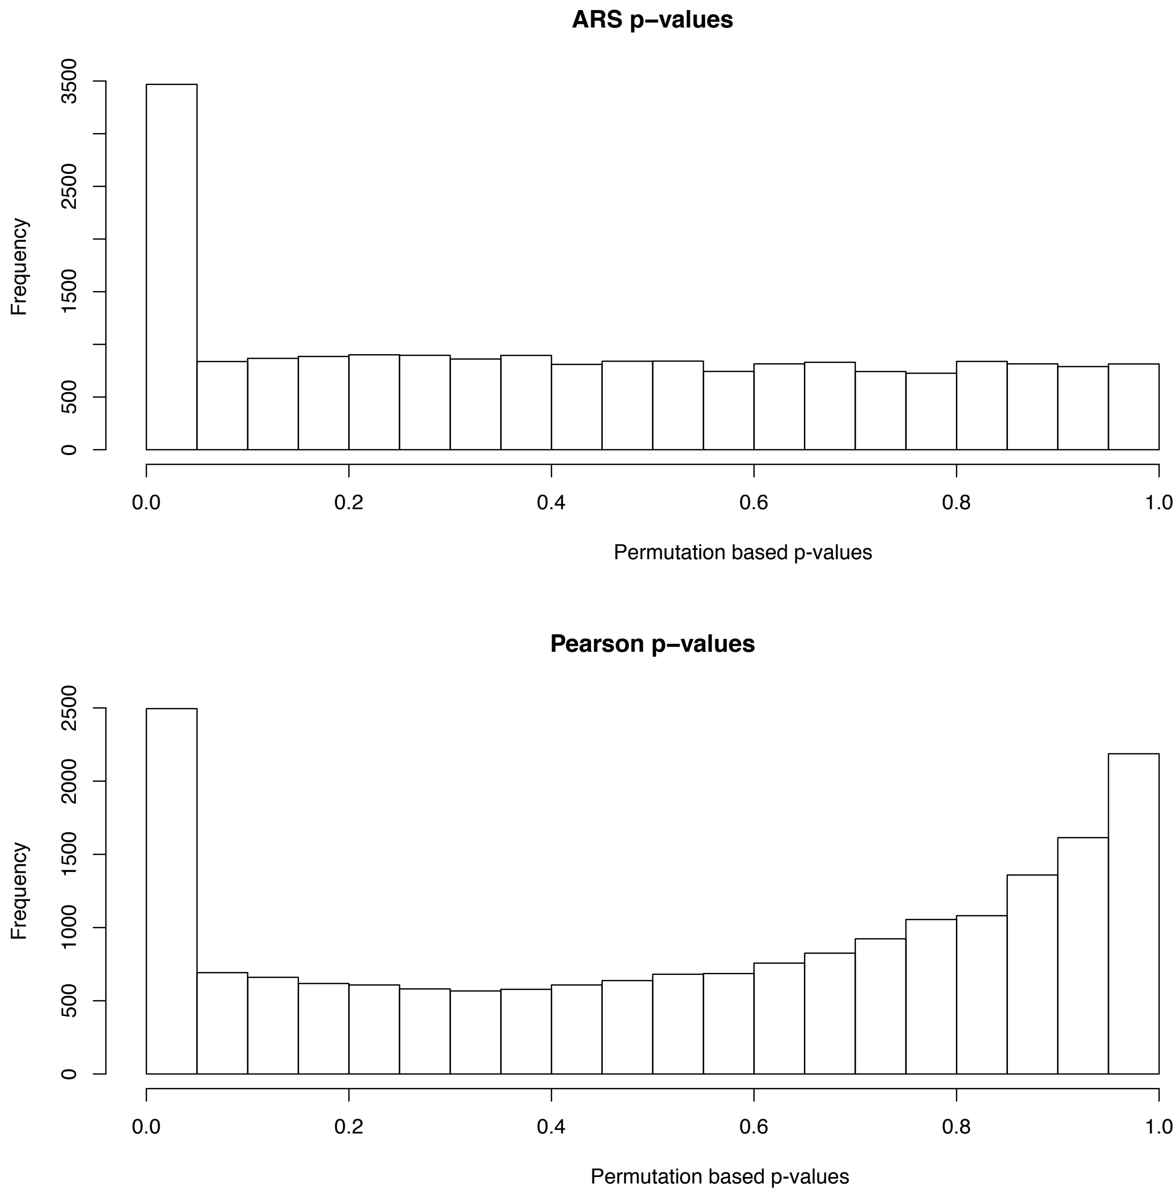


Figure S4: **Comparison of p-values obtained from randomized null data with ARS and Pearson correlation.** Using the randomization algorithm on the data 100 times, we calculated permutation based p-values for both ARS statistics and Pearson correlations. ARS generates well-behaved p-values (e.g., p-values $> 0.5$ are Uniform), while Pearson correlation results in a bimodal histogram since the Pearson correlation statistic is not designed for the signal in these data.

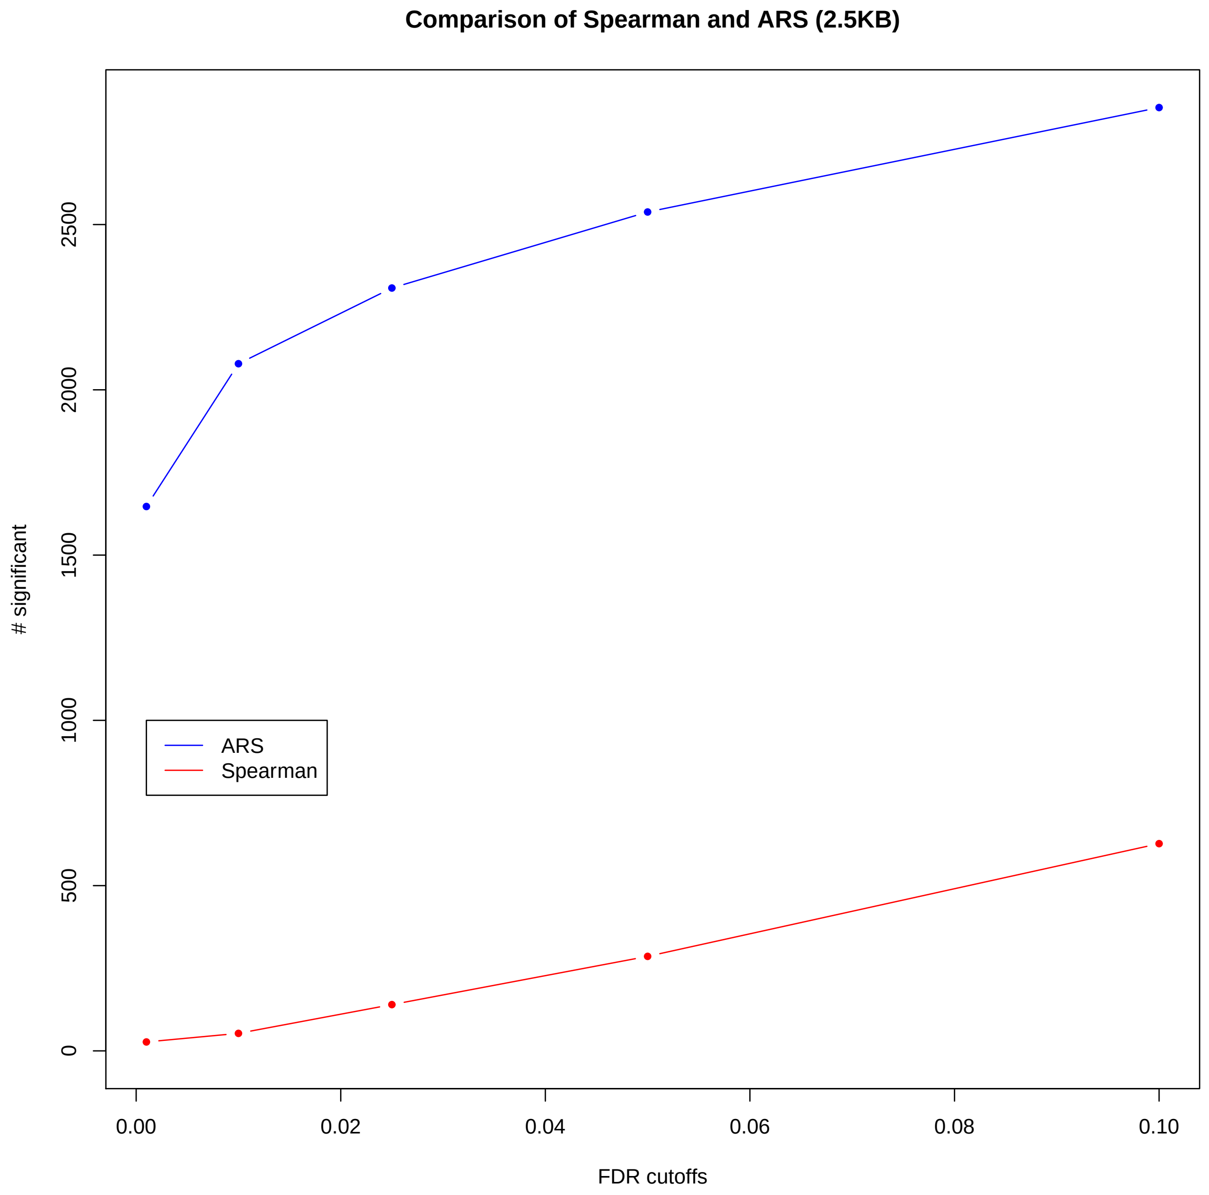


Figure S5: **Comparison of statistical significance from ARS and rank-based Spearman correlation.** Using the proximal ± 2.5kb DHS data, ARS shows superior performance relative to the rank based Spearman correlation. At given FDR thresholds, the ARS method identifies many more significant genes.

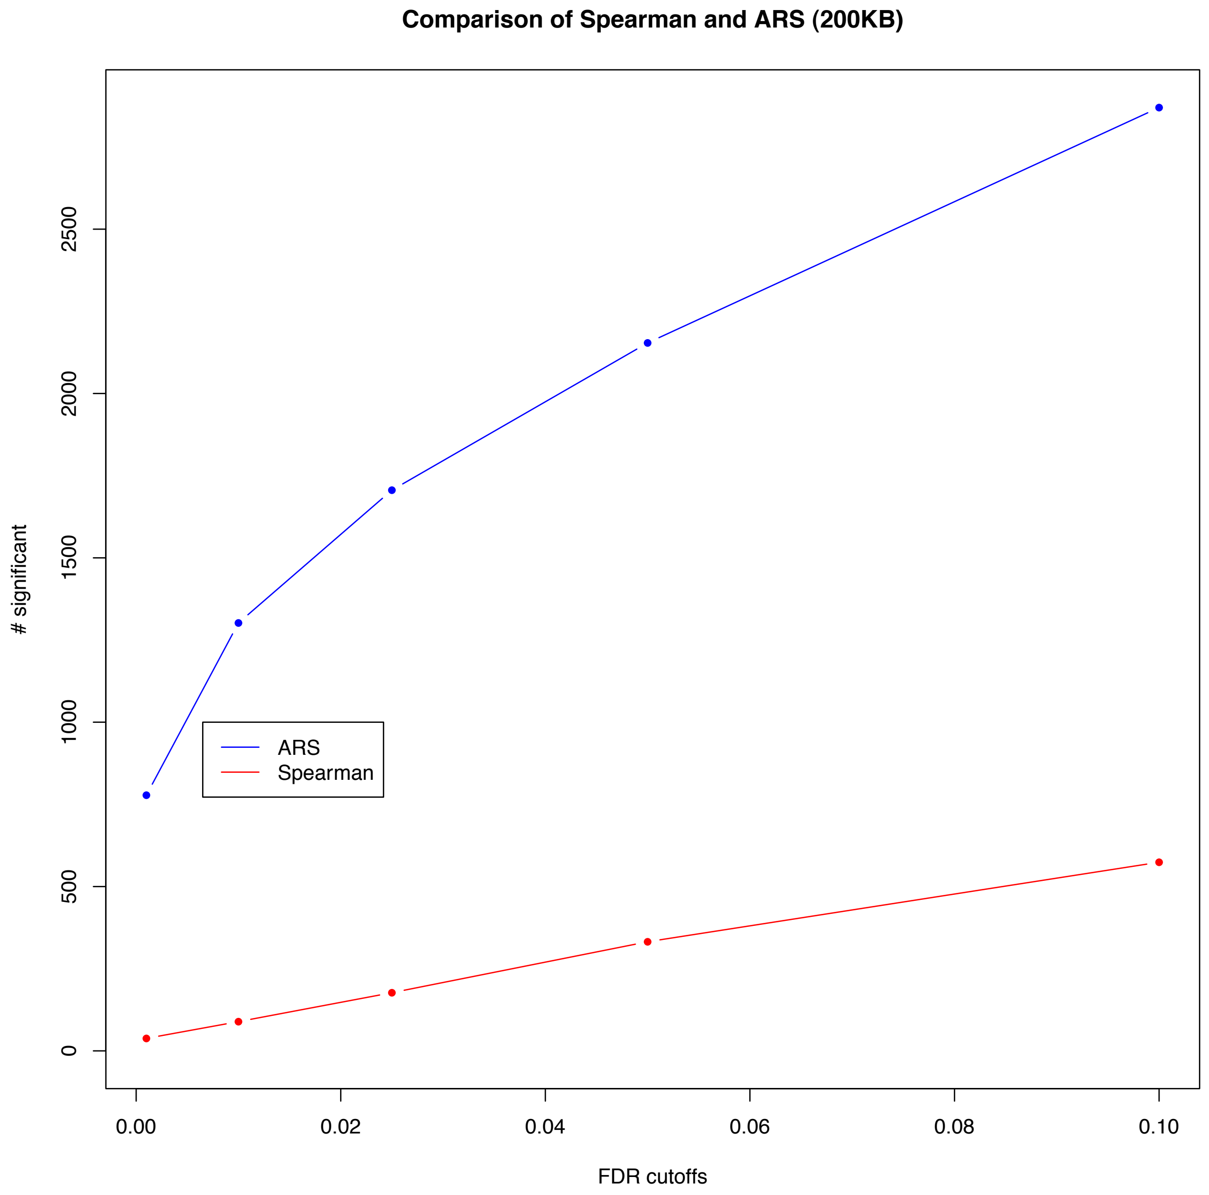


Figure S6: **Comparison of statistical significance from ARS and rank-based Spearman correlation.** Using the proximal ± 200kb DHS data, ARS shows superior performance relative to the rank based Spearman correlation. At given FDR thresholds, the ARS method identifies many more significant genes.

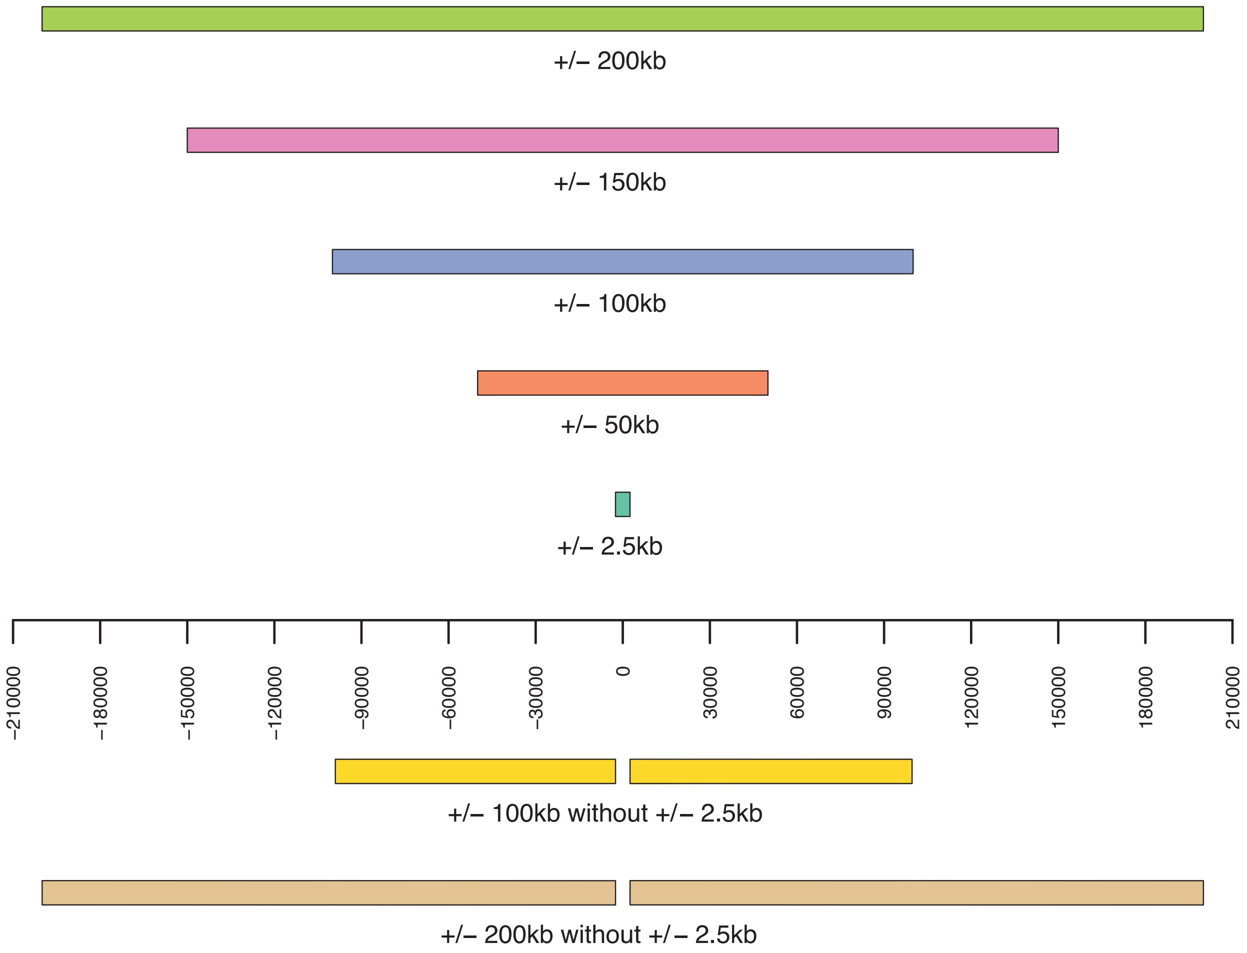


Figure S7: **Genomic segments for DHS volume.** Integrated DHS measurements across increasingly larger genomic segments relative to the TSS of the gene of interest were used to quantify gene-specific DHS volume. All data within the segment was used irrespectively of adjacent genes etc.

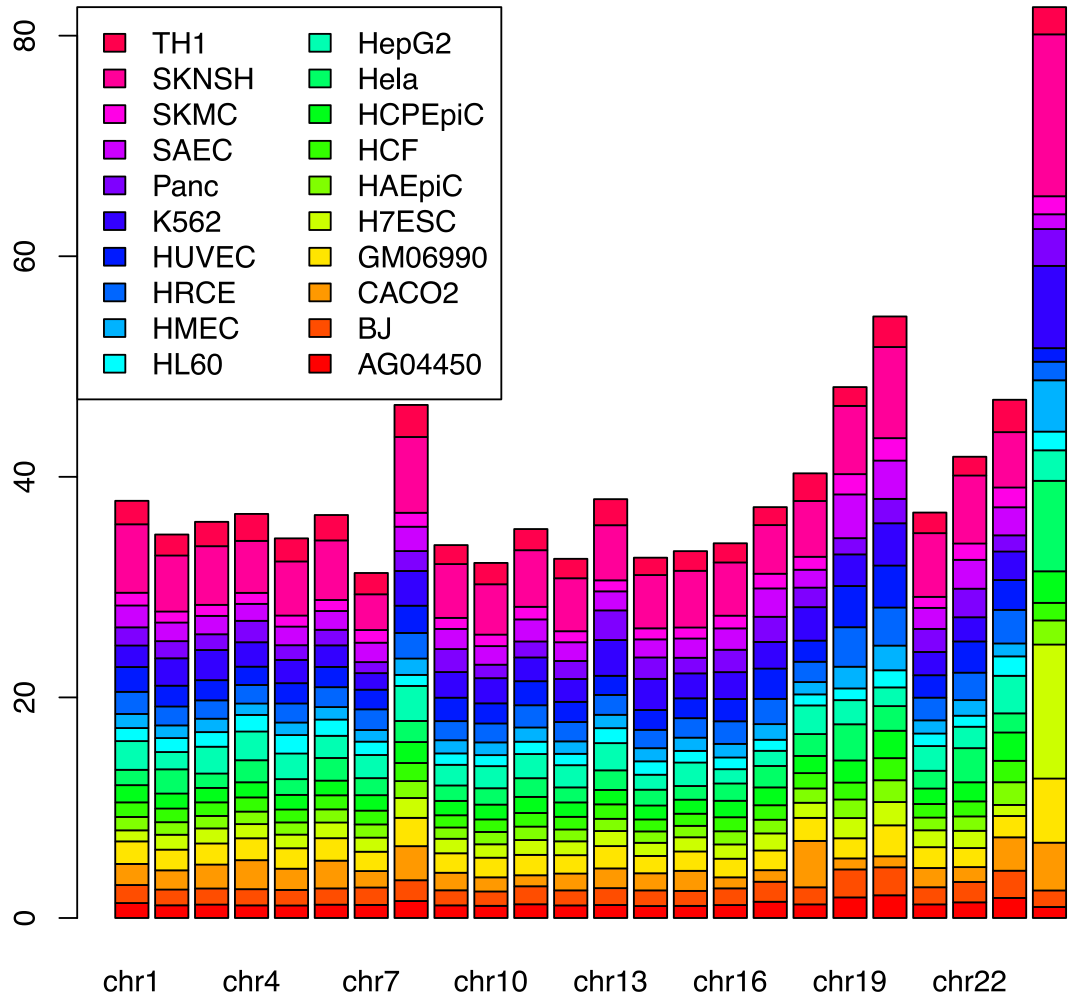


Figure S8: **Chromosome arm scaling factors.** To account for copy number variation difference in read density, etc., each DHS volume was scaled such that the total DHS volume per chromosomal arm was constant across cell-types. The above show the scaling parameter for each cell-type by chromosome.

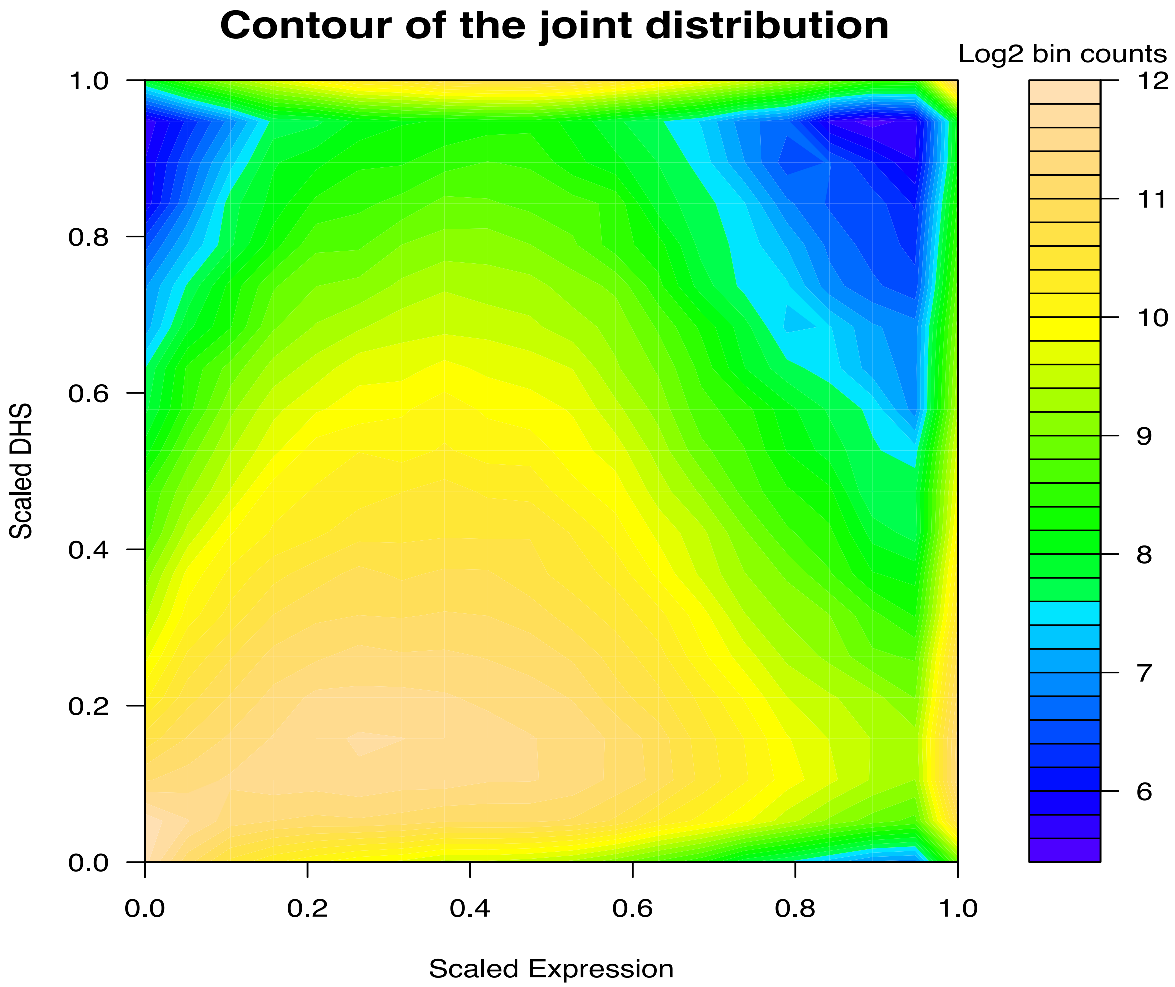


Figure S9: **Distribution of scaled data.** By scaling the DHS volume and gene expression by their per gene maximum observations and median centered, it is evident that most data points inhabit a fan-like pattern which forks away from the diagonal. Points away from the diagonal were penalized by an angular decay rate. Colors indicate $\log_2$ of the bin counts, and data were counted on a $20 \times 20$ grid.

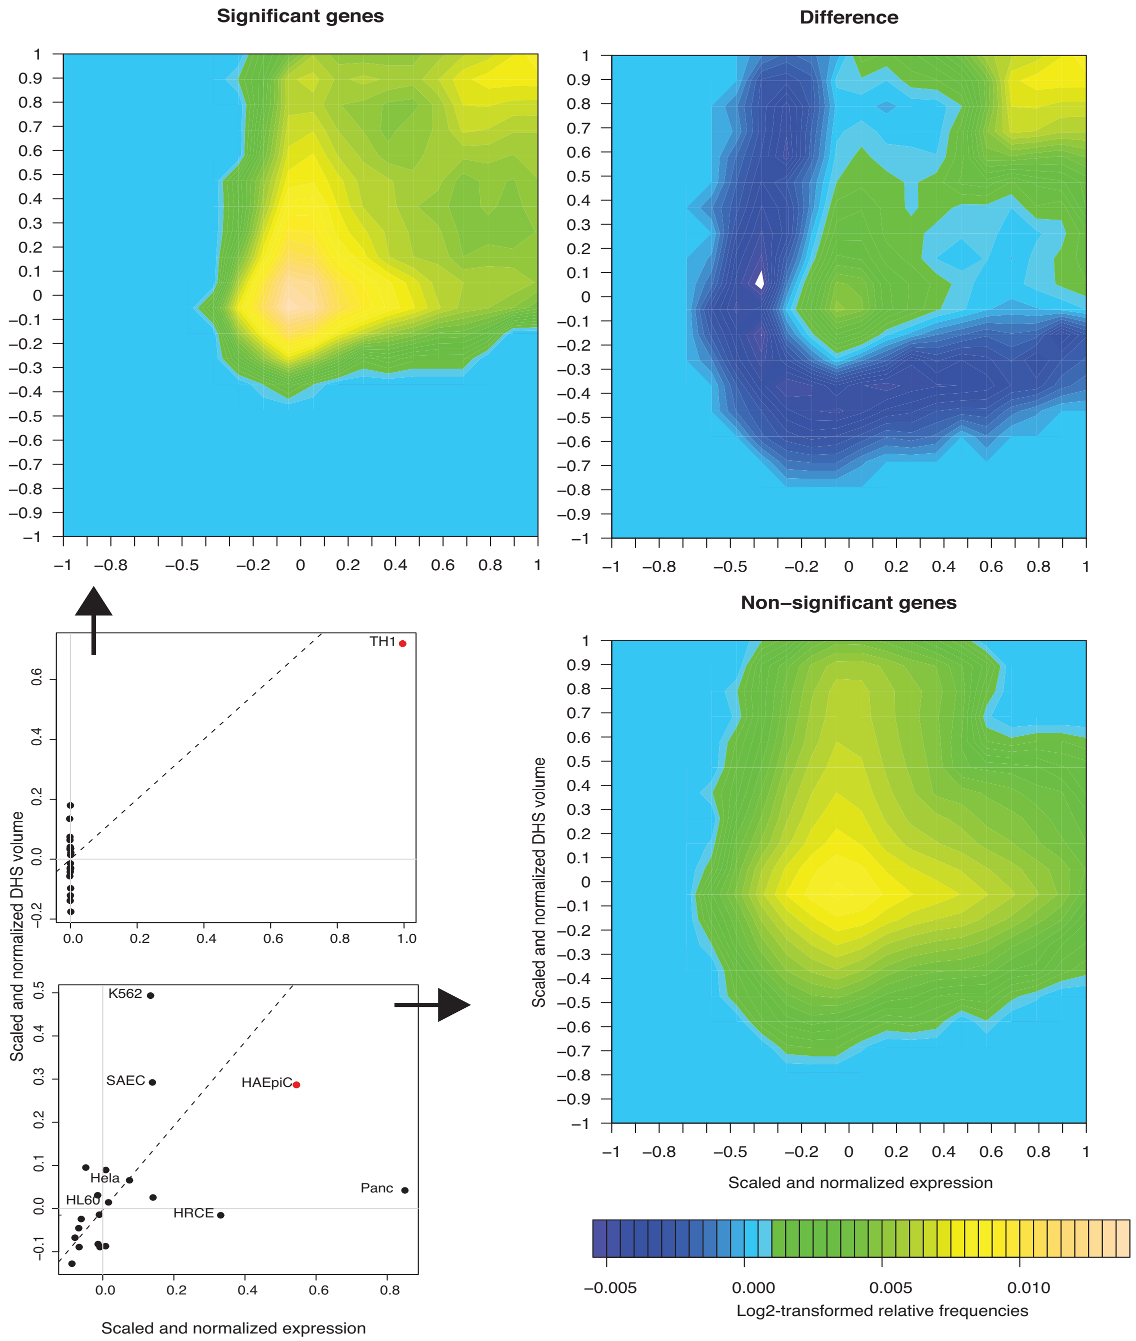


Figure S10: **Distribution of scaled and median centered data.** Scaled and median centered data for significant genes, non-significant genes, and their difference, where the color indicates the spatial distribution of points. Here, the definition of significance is determined by FDR<0.05. All x-axes display scaled and median centered expression, all y-axes display scaled and median centered DHS volume. Significant genes tend to have maximum values in both dimensions, and inhabit the upper right corner at (1,1).

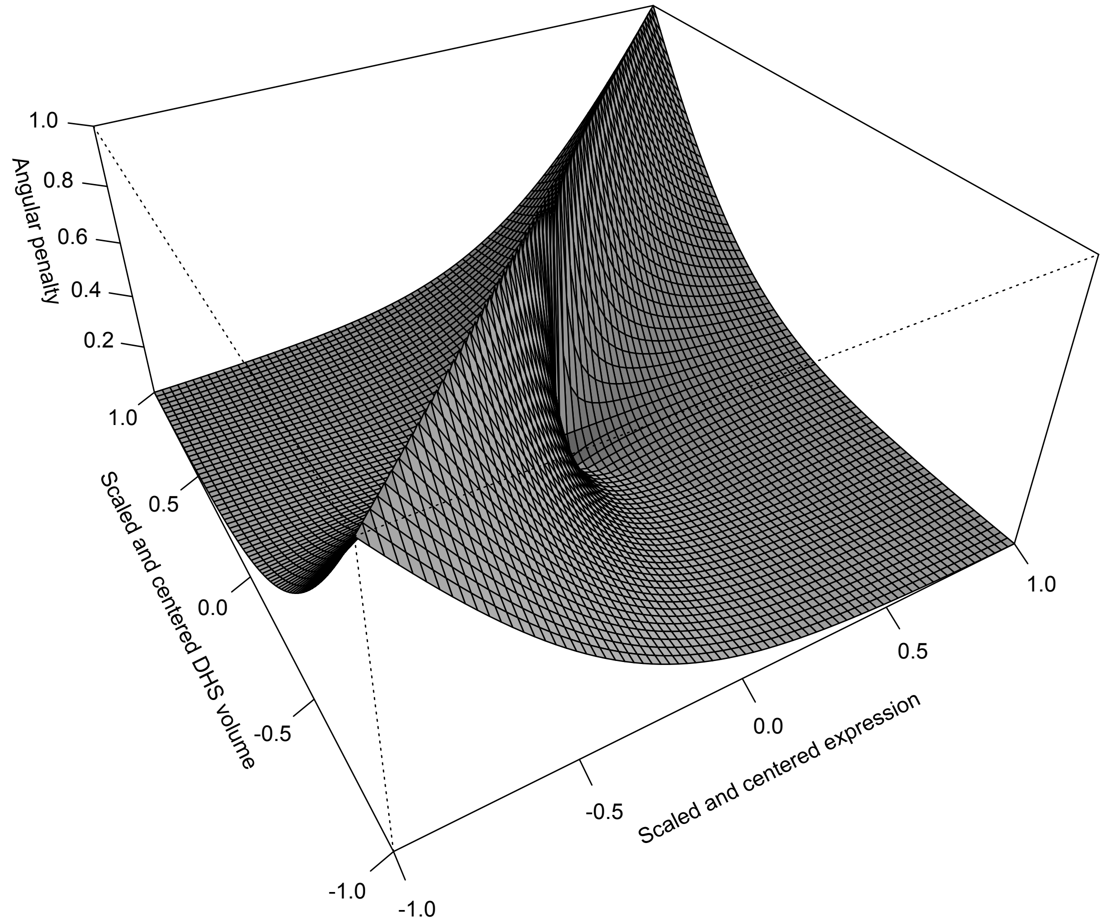


Figure S11: **Angular penalty.** A plot of the angular penalty applied to the scaled and center data. The x-axis and y-axis correspond to expression and DHS volume, and the z-axis to the angular penalty applied to any data point at the corresponding $(x, y)$ location. It can be seen that points falling along the 45° identity line are not penalized, and that the farther a point is from the line the more it is penalized.

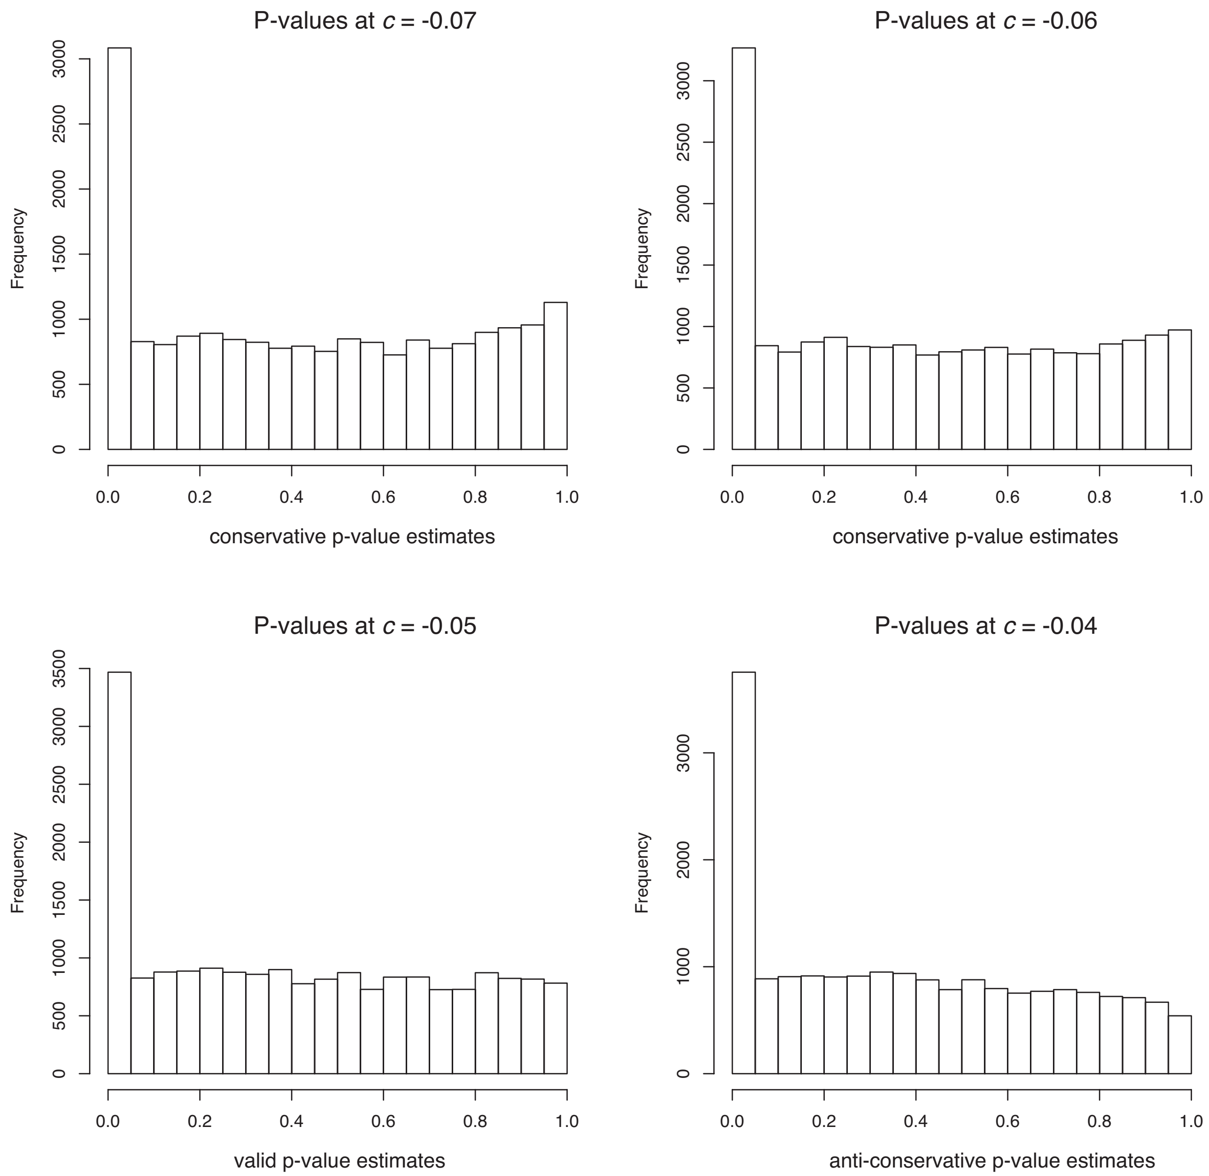


Figure S12: **The influence of $c$ on the p-value histograms.** In cases where the angular distribution is not correctly captured by $c$, the estimated p-values would either be conservative or anti-conservative in the right tail as seen above. In the above example, a value of $c = -0.05$ gave Uniform null p-values in the interval [0.5,1] according to a Kolomogorov-Smirnov test. For the presented analyses a range of values of $c$ was tested (see Figure S13), if multiple values of $c$ gave rise to Uniform null p-values the value of $c$ with the largest p-value was chosen. Due to differences in the distribution of the DHS values, values of $c$ were slightly different depending on the genomic segment investigated.

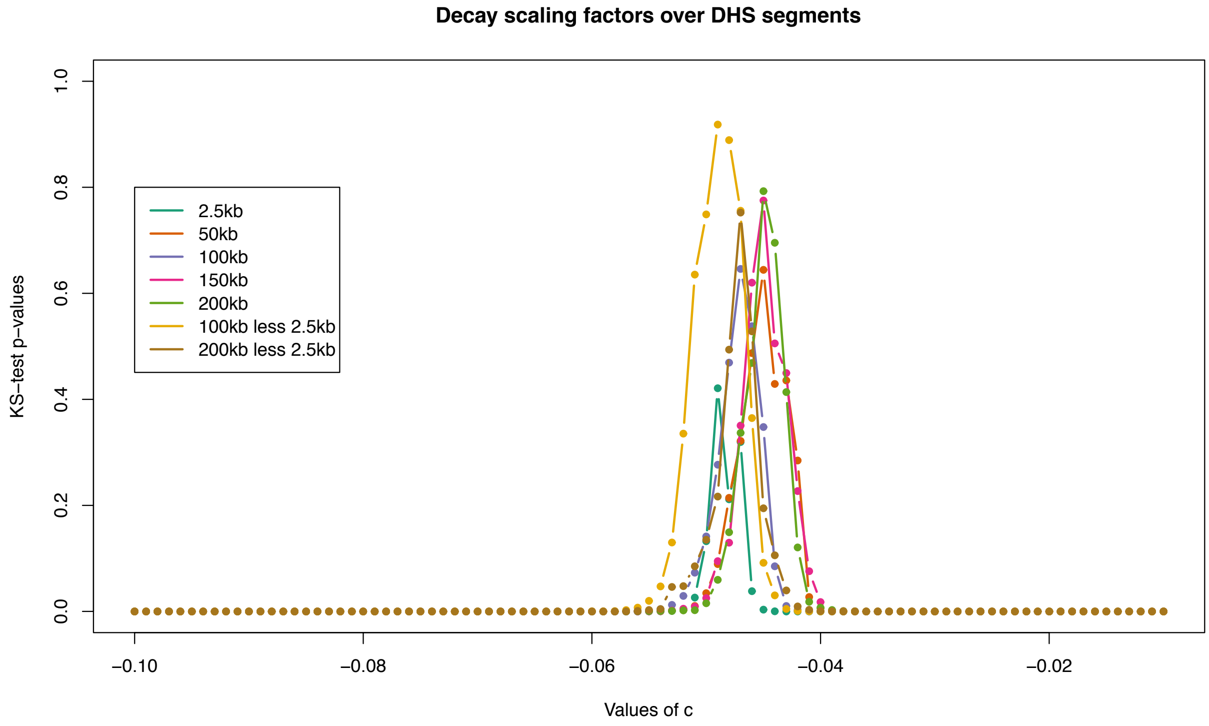


Figure S13: **Kolomogorov-Smirnov tests to determine $c$ in the angular penalty.** For each value of $c$, a Kolomogorov-Smirnov test was performed to test for Uniform null p-values defined as p-values in the interval [0.5,1]. A non-significant p-value indicates a valid choice for $c$. It can be seen that all DHS segment sizes yielded similar valid $c$ values. If multiple values of $c$ gave non-significant p-values, the value of $c$ yielding the largest p-value was chosen.

---

Figure S14 *(following page)*: **Ingenuity enrichments for biological functions**. Significant genes within the ± 100kb region found with ARS and Spearman correlation were tested for enrichment of genes with particular biological function (similar to GO-term analysis) using Ingenuity Pathways Analysis (Ingenuity Systems®, www.ingenuity.com). In general, genes called significant with ARS show a good correspondence between cell-type and the functions found enriched. Indicating that truly cell-type specific genes were indeed detected. This pattern is not as clearly seen using Spearman correlation, likely due to the fact that using correlation on this type of data leads to many false predictions.

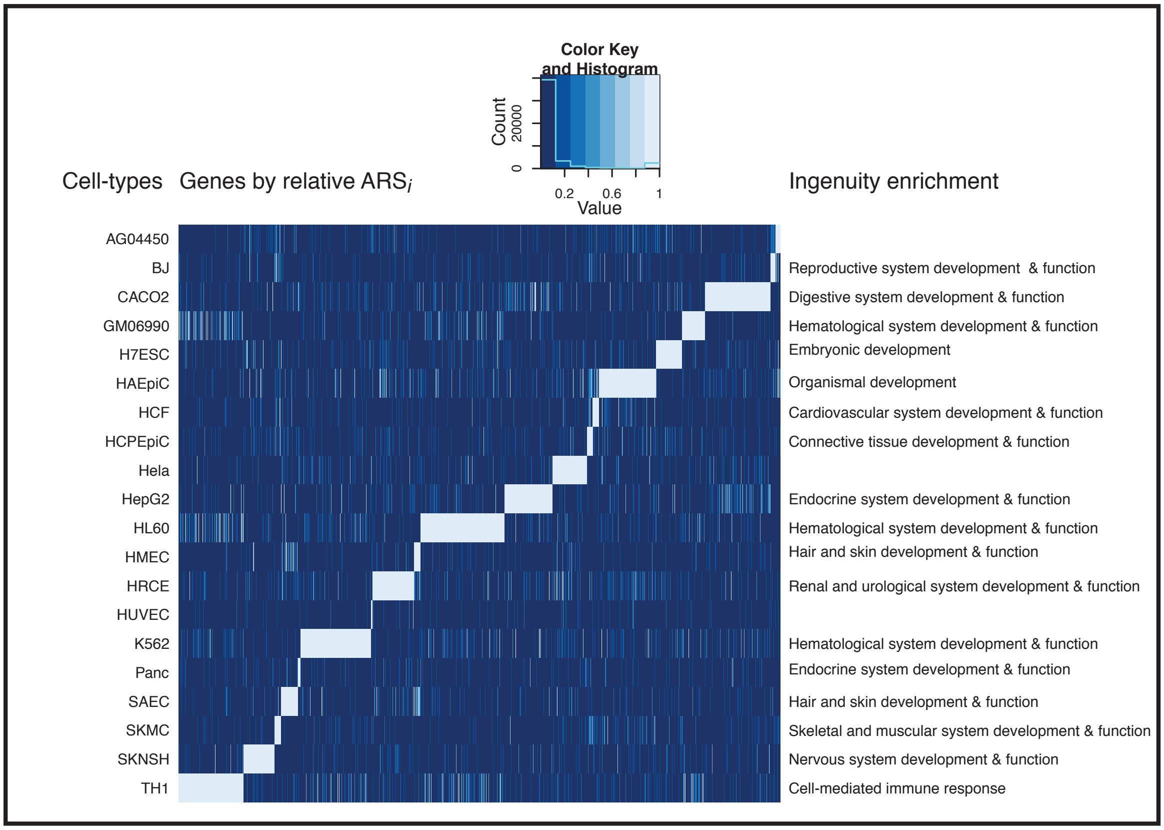
Color Key and Histogram
Count
Value
Cell-types
Genes by relative ARS$_i$
Ingenuity enrichment
AG04450
BJ
CACO2
GM06990
H7ESC
HAEpiC
HCF
HCPEpiC
Hela
HepG2
HL60
HMEC
HRCE
HUVEC
K562
Panc
SAEC
SKMC
SKNSH
TH1
Reproductive system development & function
Digestive system development & function
Hematological system development & function
Embryonic development
Organismal development
Cardiovascular system development & function
Connective tissue development & function
Endocrine system development & function
Hematological system development & function
Hair and skin development & function
Renal and urological system development & function
Hematological system development & function
Endocrine system development & function
Hair and skin development & function
Skeletal and muscular system development & function
Nervous system development & function
Cell-mediated immune response

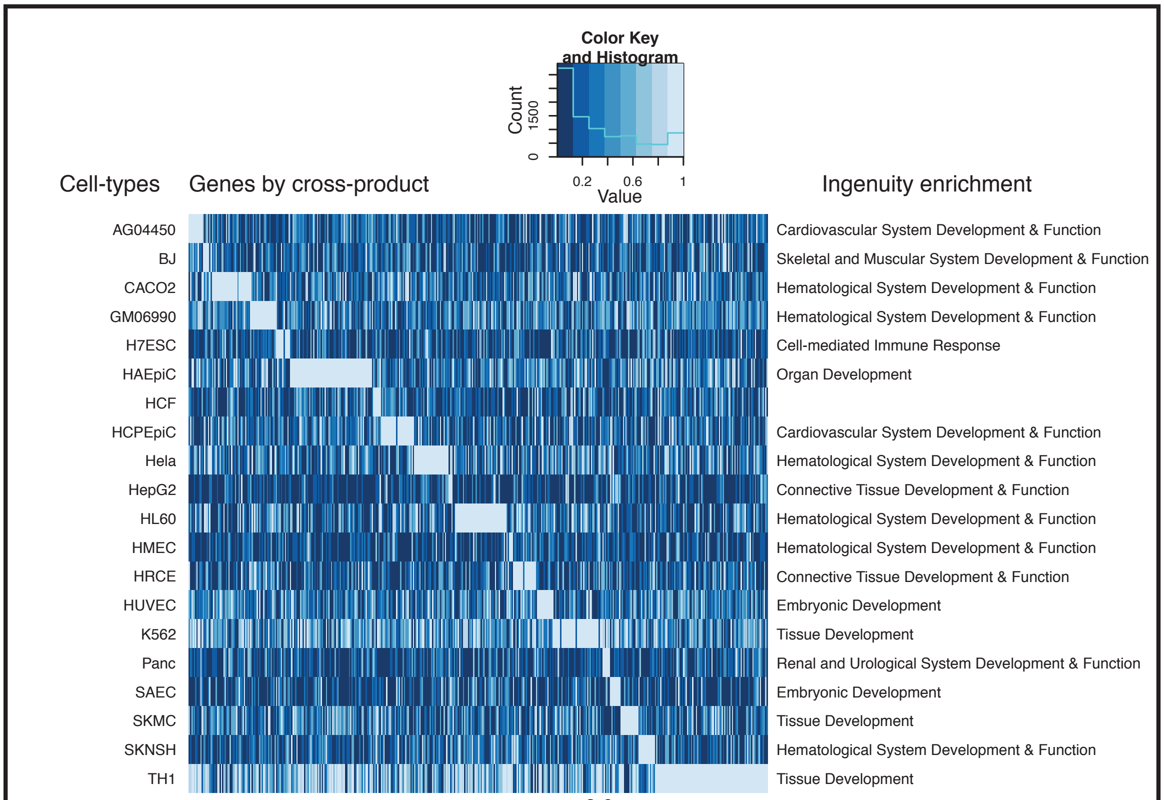
Color Key and Histogram
Count
Value
Cell-types
Genes by cross-product
Ingenuity enrichment
AG04450
BJ
CACO2
GM06990
H7ESC
HAEpiC
HCF
HCPEpiC
Hela
HepG2
HL60
HMEC
HRCE
HUVEC
K562
Panc
SAEC
SKMC
SKNSH
TH1
Cardiovascular System Development & Function
Skeletal and Muscular System Development & Function
Hematological System Development & Function
Hematological System Development & Function
Cell-mediated Immune Response
Organ Development
Cardiovascular System Development & Function
Hematological System Development & Function
Connective Tissue Development & Function
Hematological System Development & Function
Hematological System Development & Function
Connective Tissue Development & Function
Embryonic Development
Tissue Development
Renal and Urological System Development & Function
Embryonic Development
Tissue Development
Hematological System Development & Function
Tissue Development

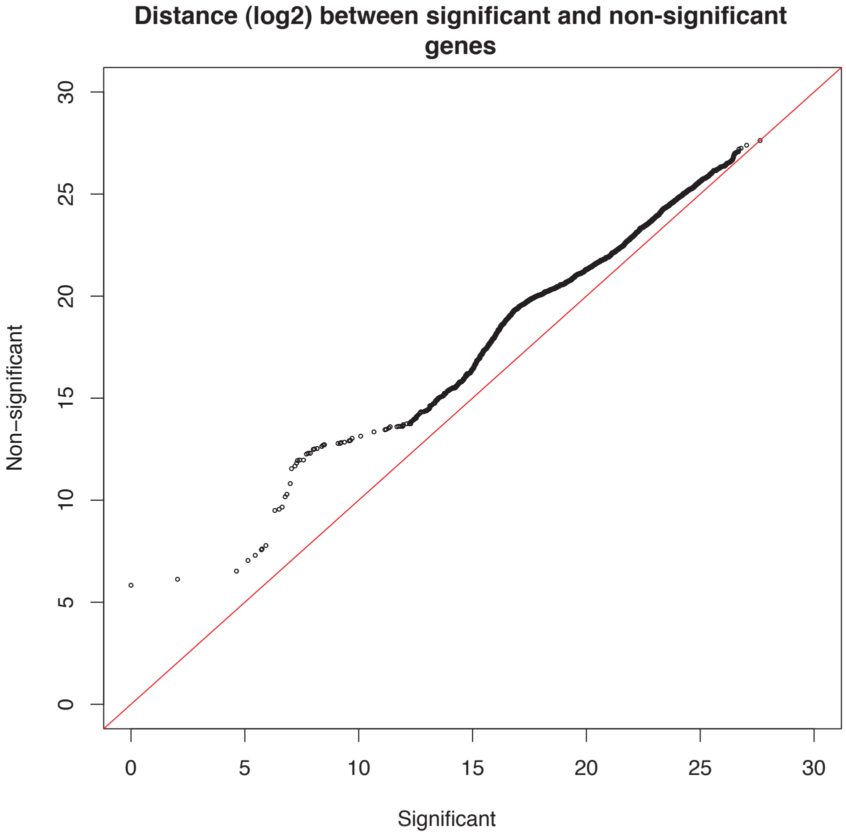


Figure S15: **Aggregation of cell-type specific genes.** Four different tests were done to test for aggregation of significant genes according to genomic location and maximal cell type. Here, the distance between significant genes are plotted against the distance between non-significant genes. The number of null genes were chosen to match the number of significant genes from that cell-type, such that the effect is not primarily driven by cell-type. A clear and significant trend show that cell-type significant genes aggregate along the genome.

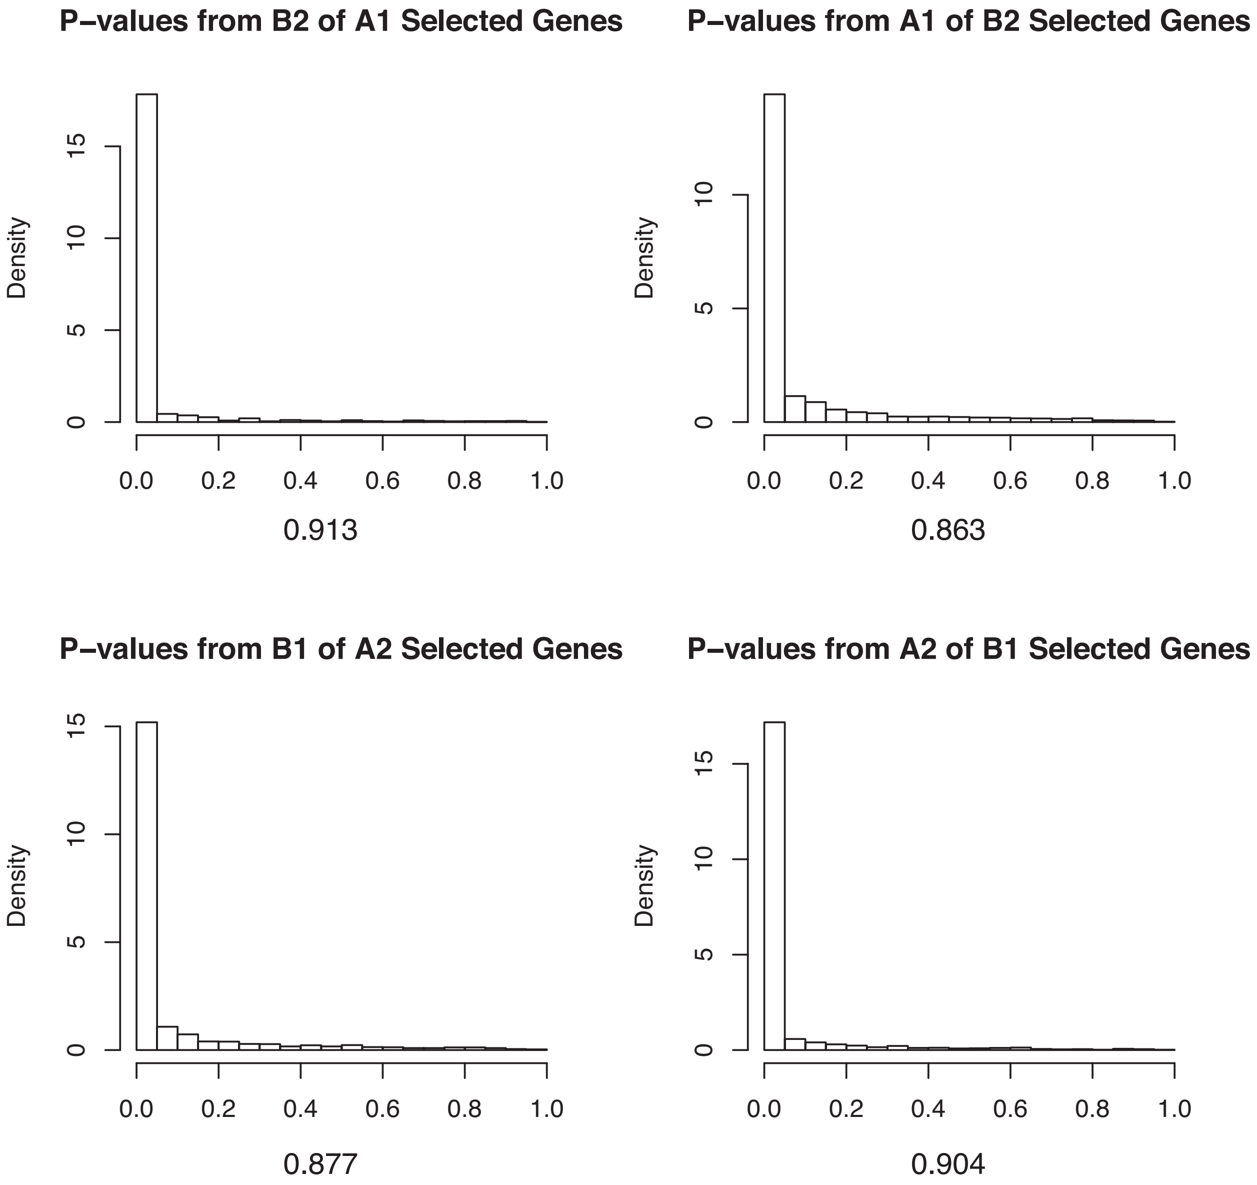


Figure S16: **Assessment of reproducibility.** The p-values corresponding to genes significant (FDR $<$ 0.05) from one DHS and gene expression replicate are plotted for the complementary analysis. It can be seen that small p-values from one data set yield small p-values from the replicated data set, indicating a high level of reproducibility. The fraction recaptured at FDR$<$0.05 is listed below each histogram.

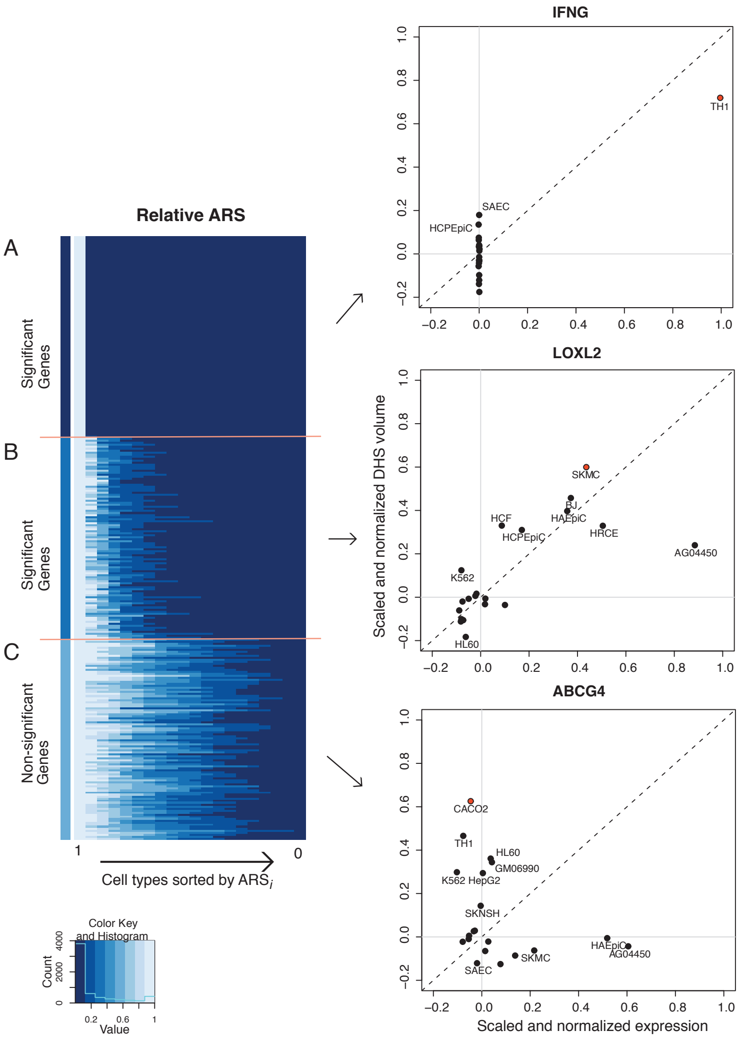


Figure S17: **Relative ARS scores.** For each gene we can scale the $\text{ARS}_i$ values by $\text{ARS}_{\text{max}}$ in order to distinguish between significant genes with an "on-off" effect and significant genes which show a more gradual trend (i.e., more than a single cell-type may act as an outlier compared to the remaining cell-types). Significance is here determined as FDR $< 0.05$. In the color image cell-types are sorted, column-wise, by decreasing scaled $\text{ARS}_i$, the image is further divided into three blocks, representing the three major distributions of $\text{ARS}_i$ observed. (A) Significant genes with a singular outlier, i.e. "on-off", (B) significant genes with a gradual trend, and finally (C) non-significant genes with no distinct outliers as can be seen from the high relative $\text{ARS}_i$ values extending across multiple cell-types. Right of each sub-panel is a 2D plot of the scaled and centered gene expression by DHS volume showing a representative gene from the given distribution: *IFNG*, *LOXL2*, and *ABCG4* respectively.

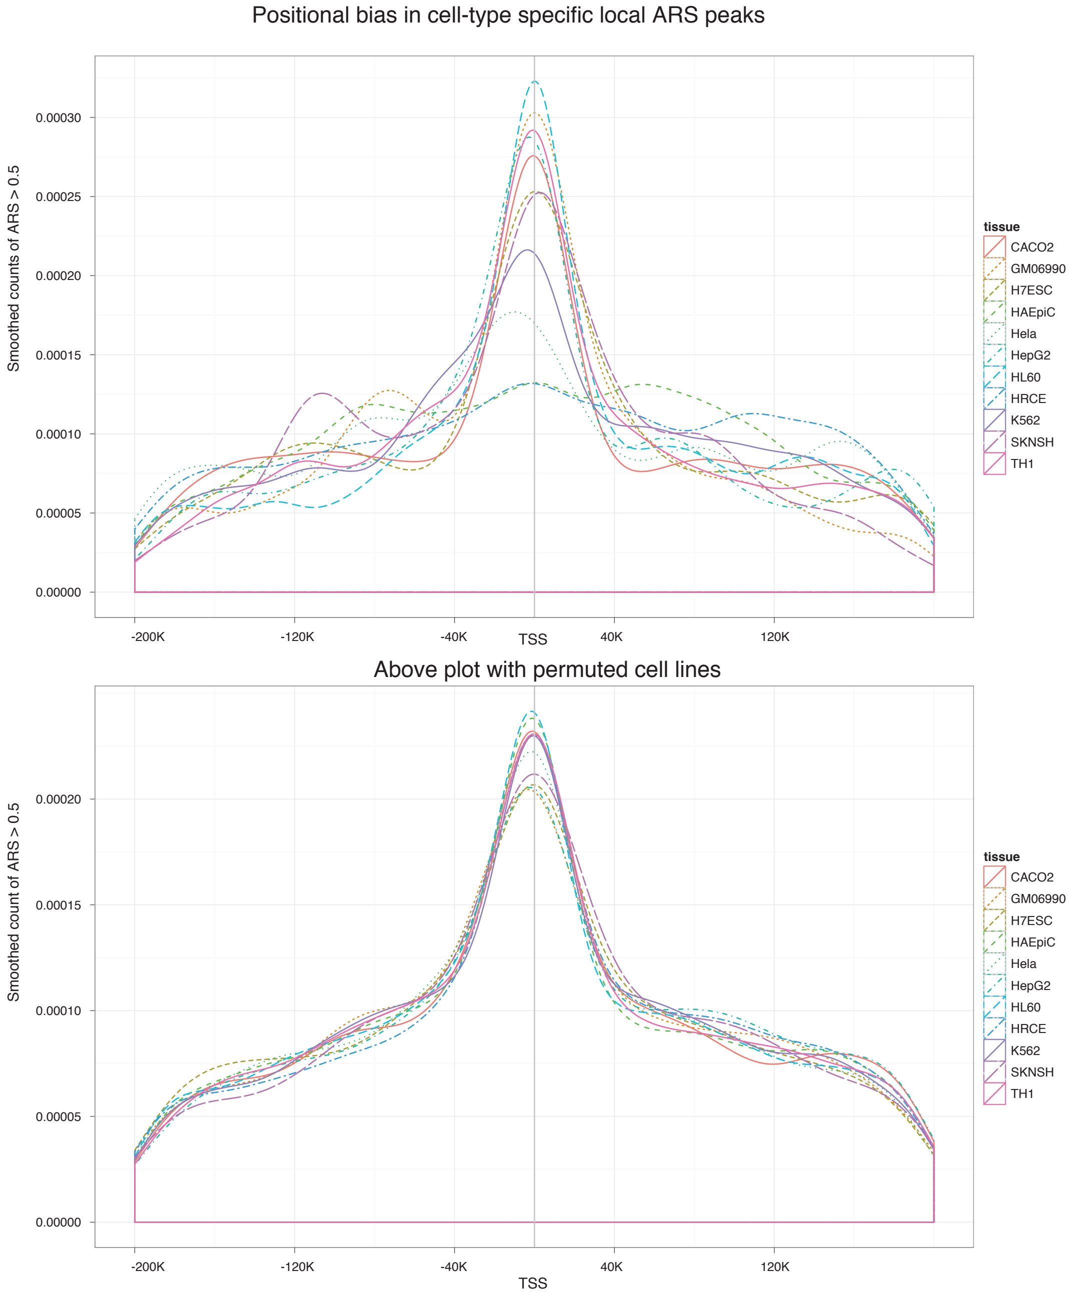


Figure S18: **Positional densities of local ARS peaks by cell-type** The positional bias of cell-type specific local ARS peaks can be seen in the upper panel. For example, HL60 shows a more proximal signal relative to that of HAEpiC. A clear difference in the amount of distal regulation is seen across the different cell-types. The lower panel shows the same analysis applied to the data where the cell types are randomly shuffled among the cases considered in the upper panel.

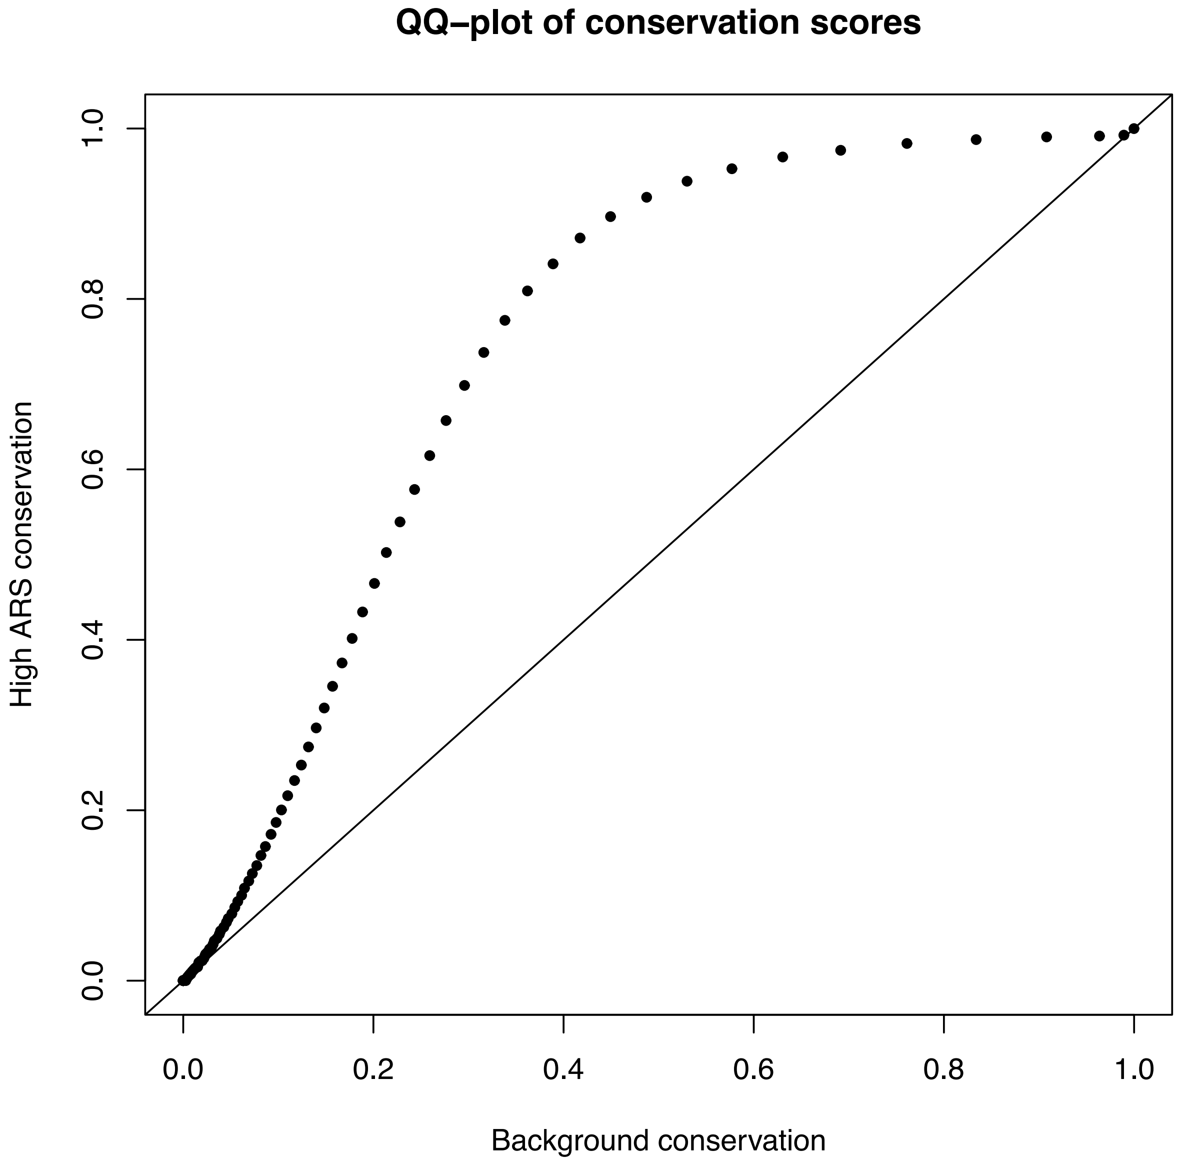


Figure S19: **Conservation of sequences corresponding to local ARS peaks.** Phastcons scores within local ARS peaks and a negative control set were recorded and displayed in the quantile-quantile plot. The local ARS peaks show a marked and significantly (Kolmogorov-Smirnov p-value $< 2.2e\text{-}16$) higher conservation relative to the negative control set, indicating that local ARS peaks are strong candidates for functional regions.

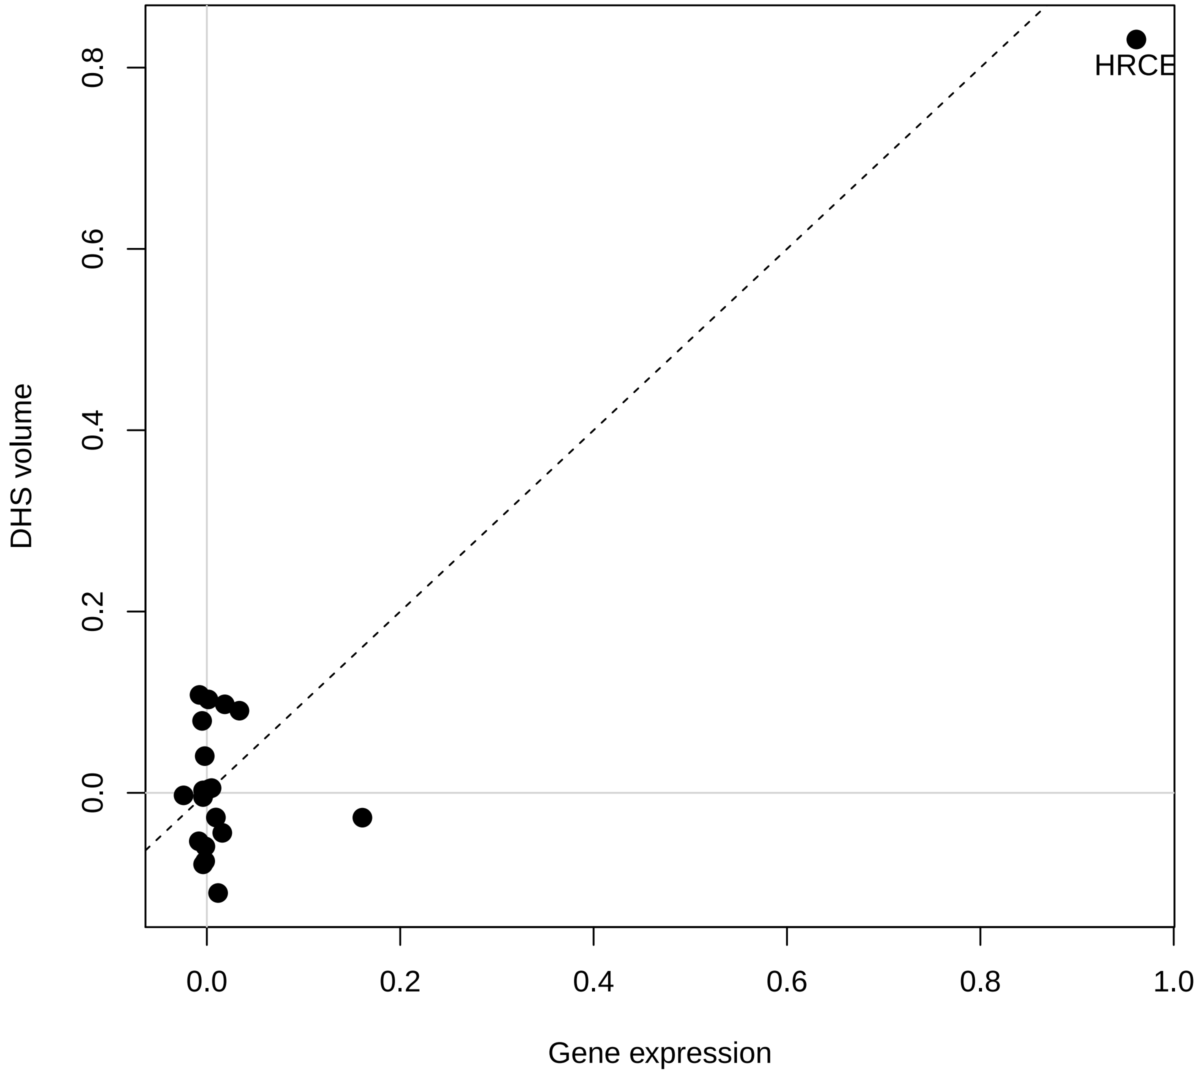


Figure S20: ***HNF1B* as chromatin / gene expression concordant in HRCE.** While genes significant in HRCE have a clear over-representation of the *HNF1B* motif, the gene itself is also in chromatin / gene expression concordance.

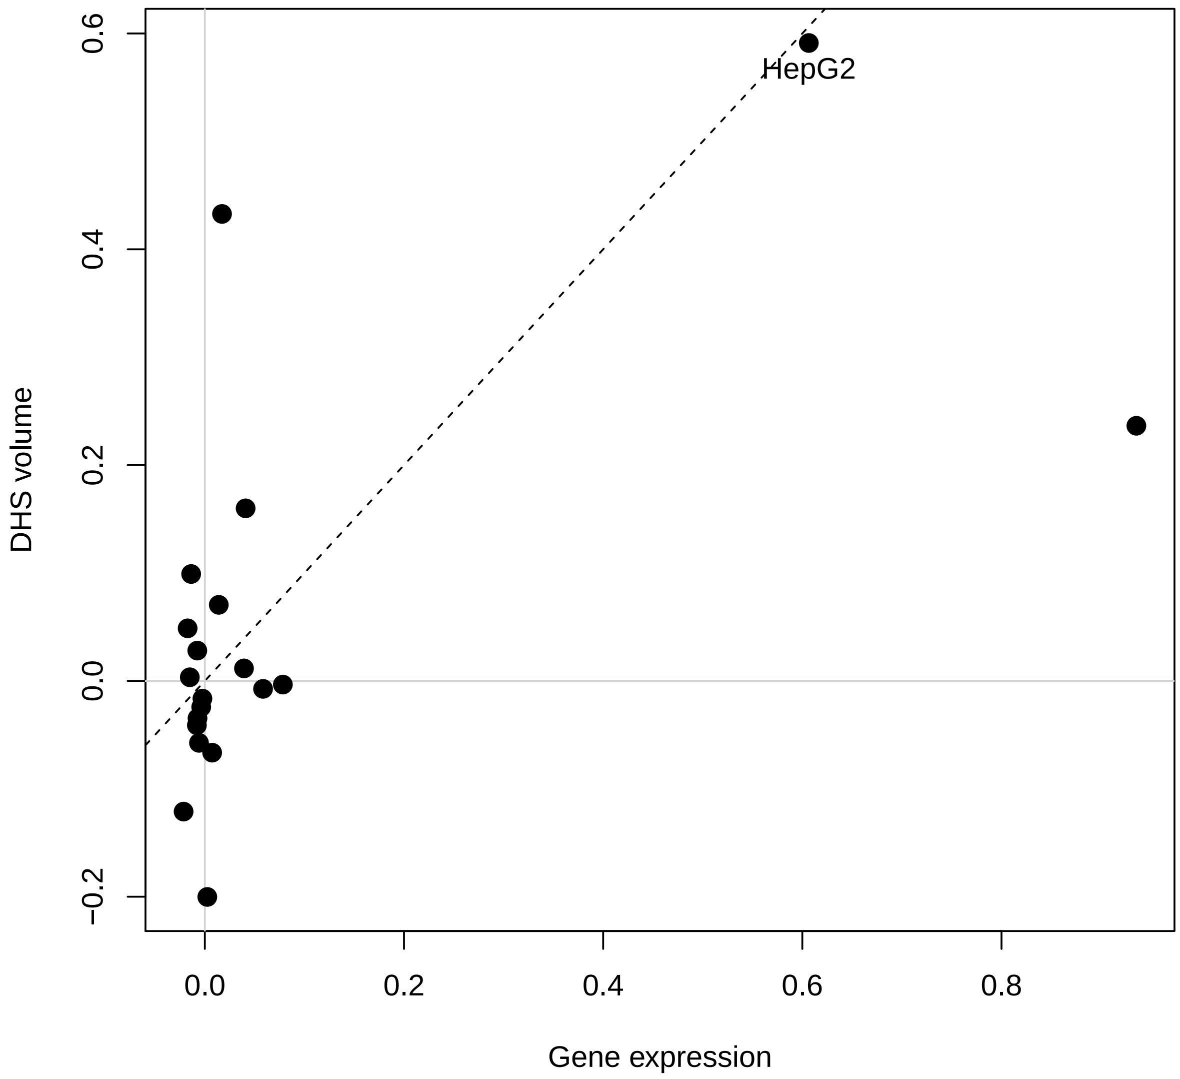


Figure S21: ***HNF4A* as chromatin / gene expression concordant in HepG2.** While genes significant in HepG2 have a clear over-representation of the *HNF4A* motif, the gene itself is also in chromatin / gene expression concordance.

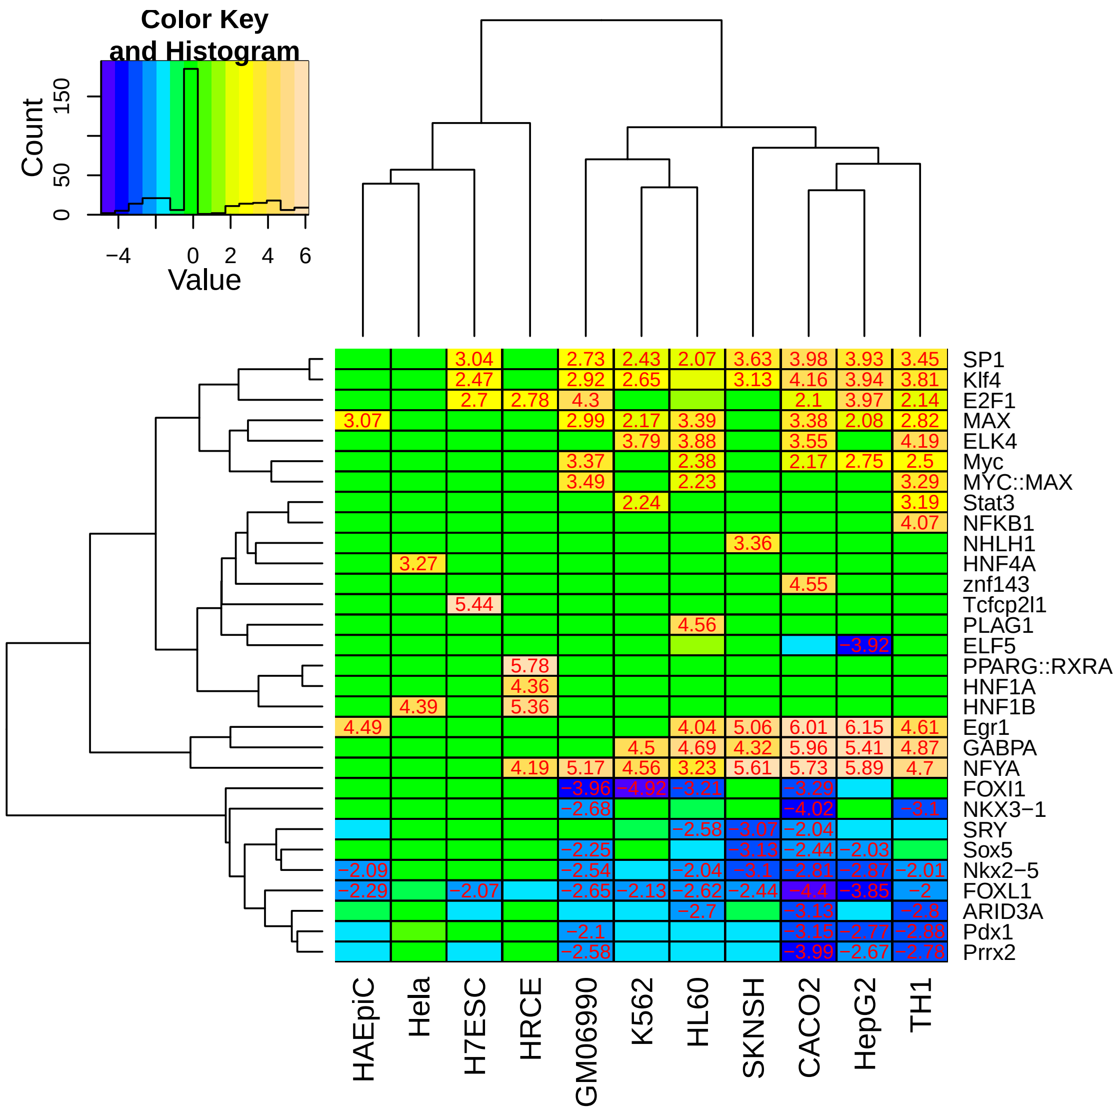


Figure S22: **Over- and under-representation of TFBS within cell-type specific proximal (±10kb) promoters.** Using only the proximal (±10kb) regions for the local ARS peak TFBS analysis, known cell-specific interactions disappear, e.g., Sox2 and Pou5f1 (Oct4) for H7ESC.

DHS across all cell-types for HBB and HBE1

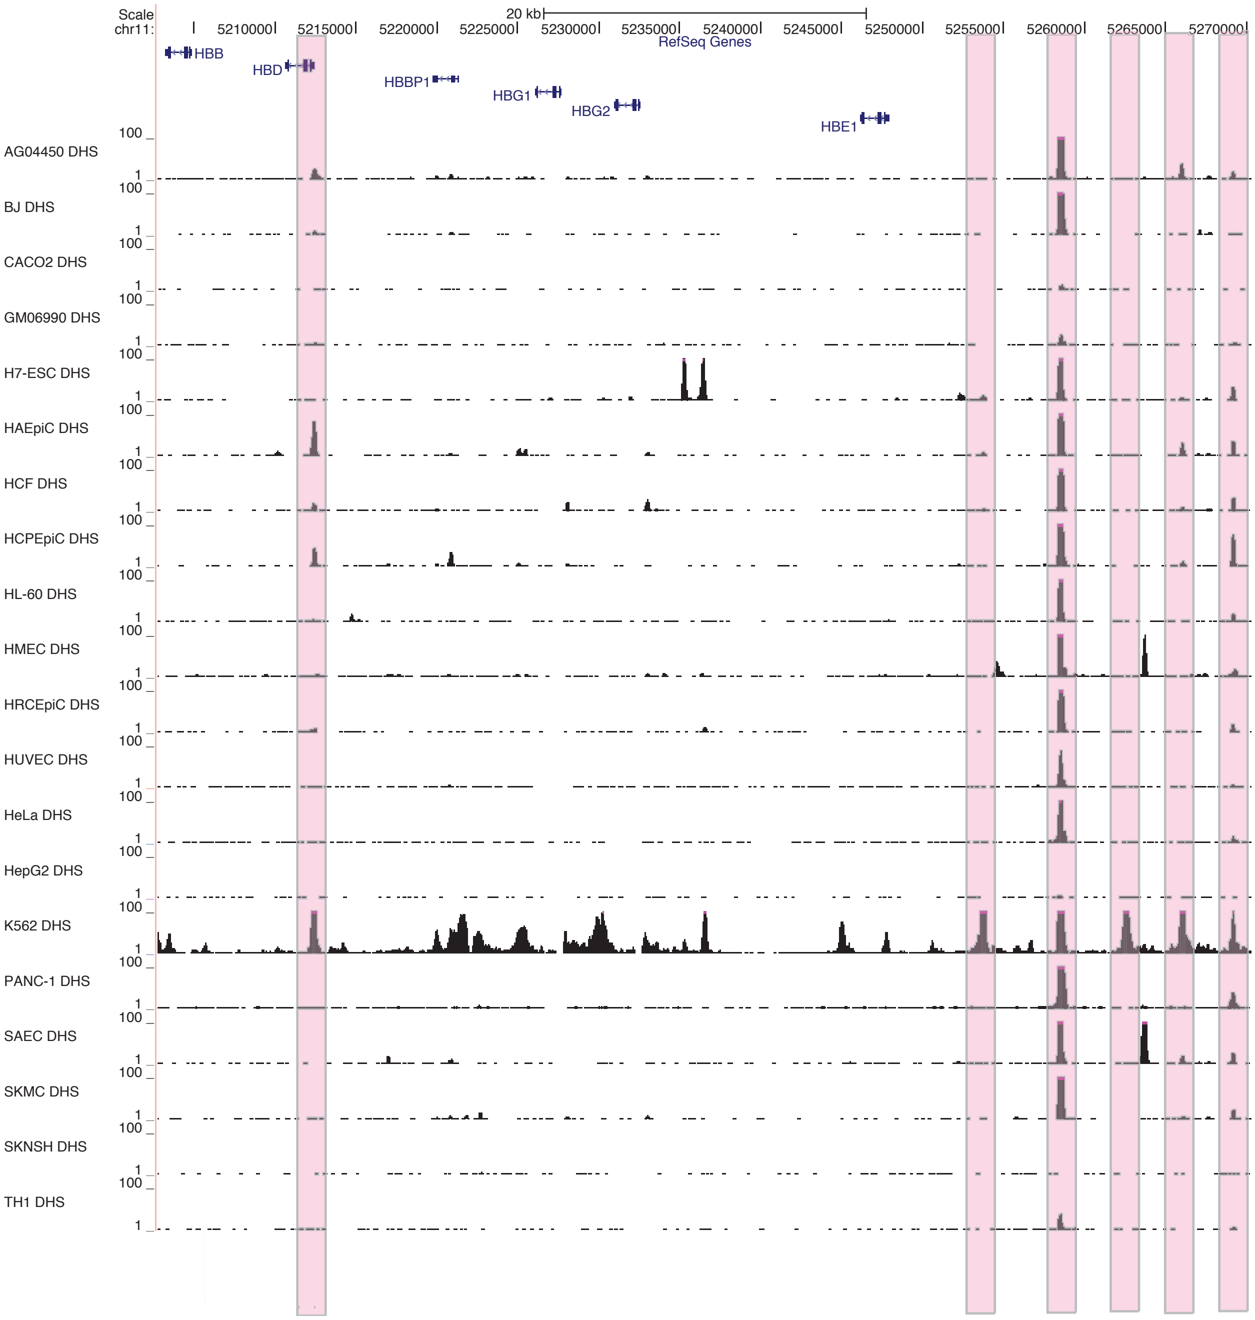


Figure S23: **Raw DHS fragments for *HBB* and *HBE1*.** The DHS values within a region of interest for *HBB* and *HBE1* across all cell-types are highlighted by salmon colored bars. These regions correspond to known hypersensitive regions. Interestingly, one region is present in almost all cell-types, whereas, others are unique to K562.

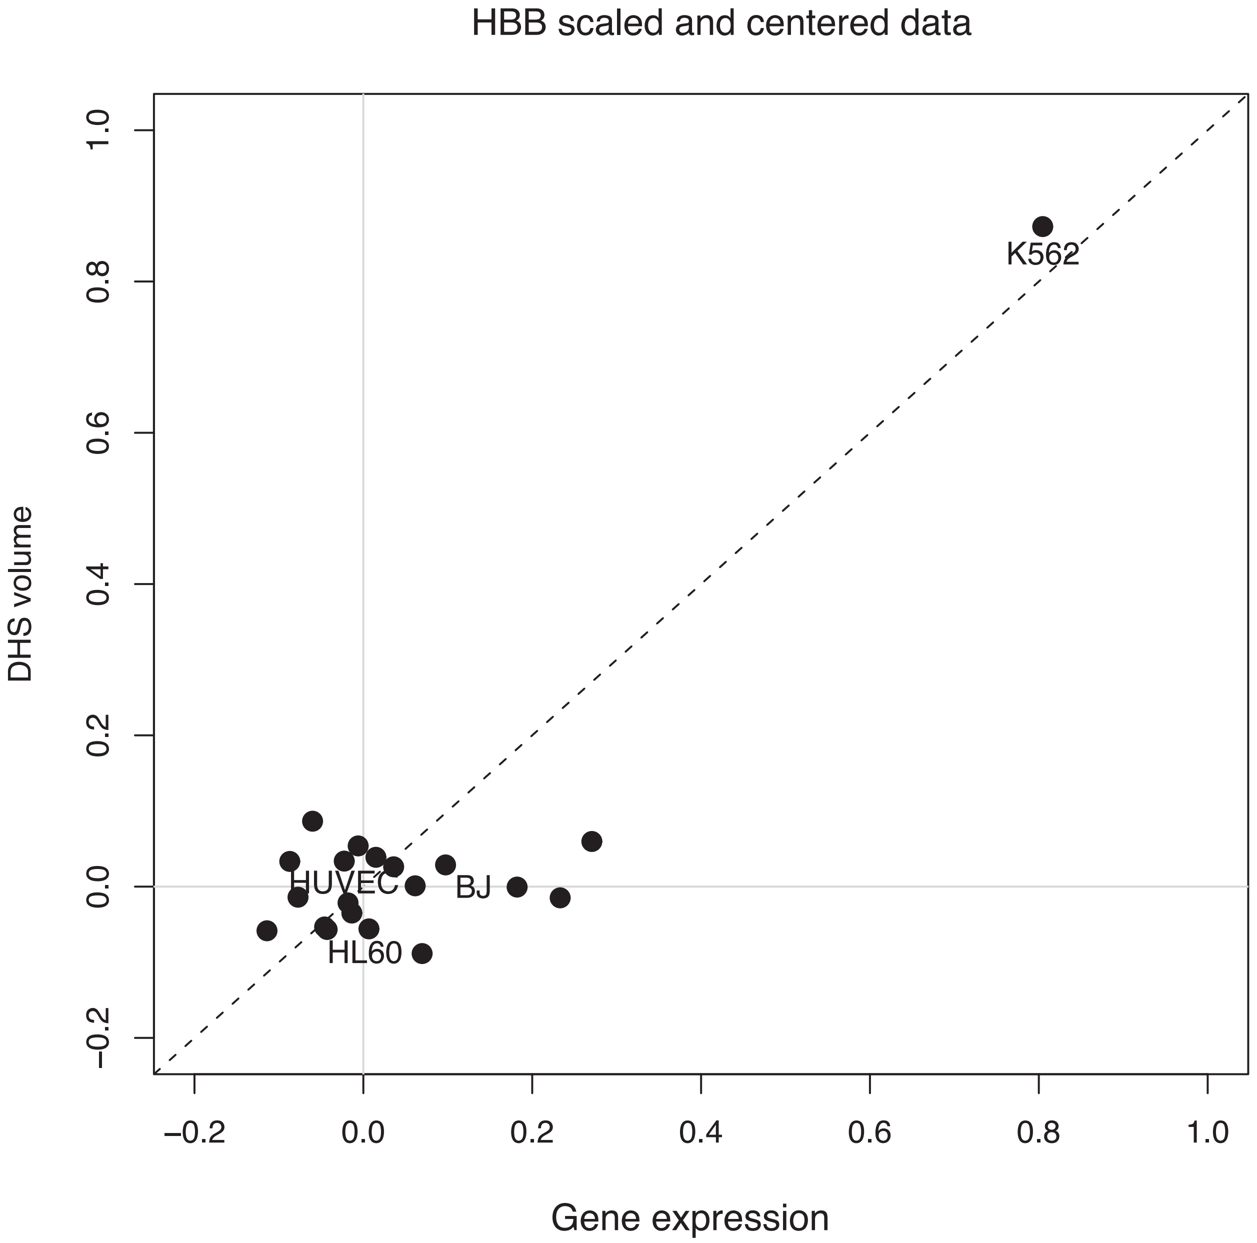


Figure S24: **Scaled and centered gene expression and DHS volume for *HBB*.** The gene expression and DHS volume [0-1] scaled and medoid centered for all 20 cell-types, across the entire ± 100kb DHS segment. This show *HBB* as a clear and singular outlier for K562.

ARS across all cell-types for HBB

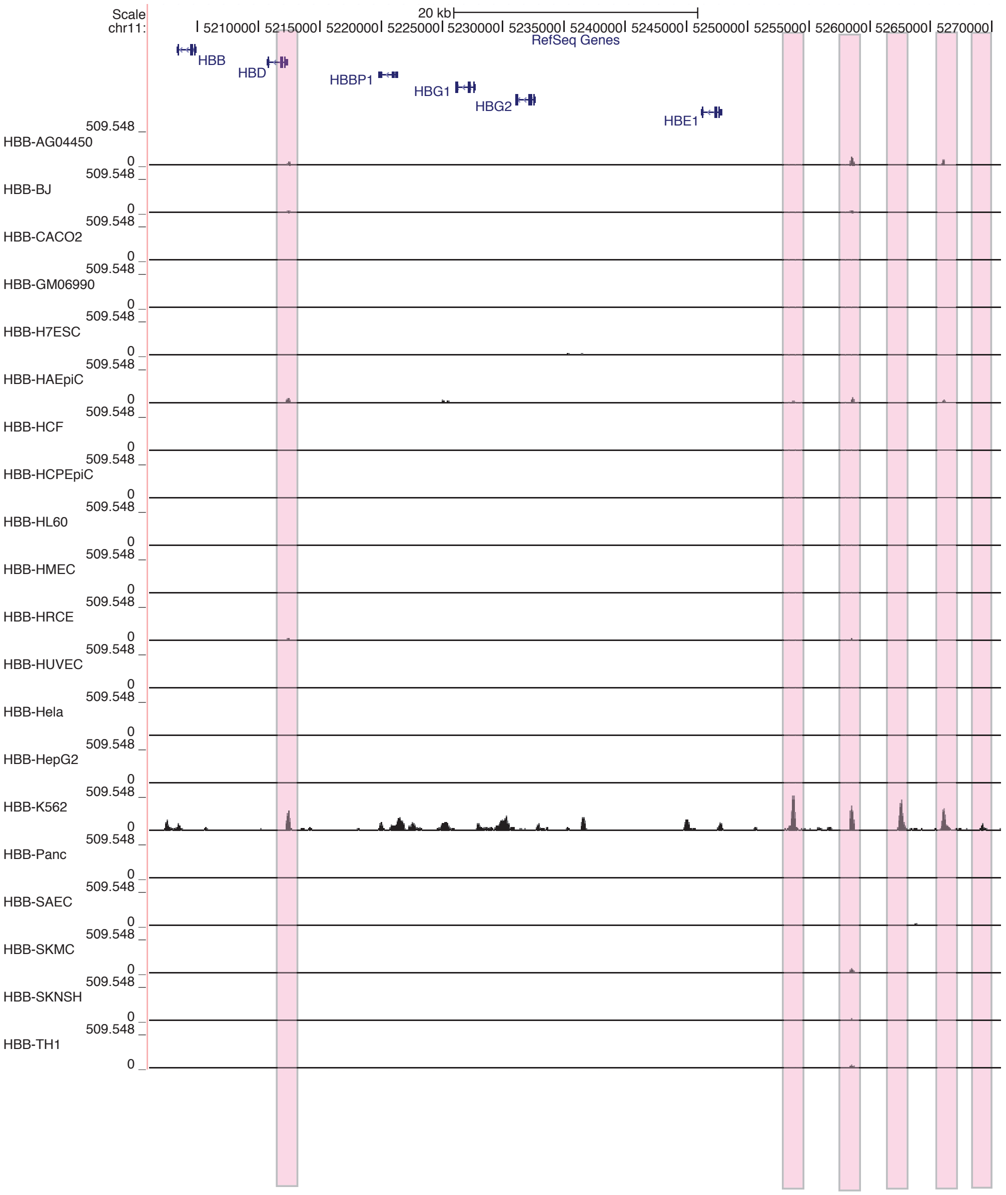


Figure S25: **ARS profiles for *HBB*.** Local ARS profiles across all 20 cell-types, where the salmon colored bars indicate ARS peaks. The 6th hypersensitive site (from the left) is not seen as an ARS peak, due to its presence in multiple cell-types. The hypersensitive site present in the 3rd bar (from the left) appears as an ARS peak, despite being present in all cell-types due to its high local value.

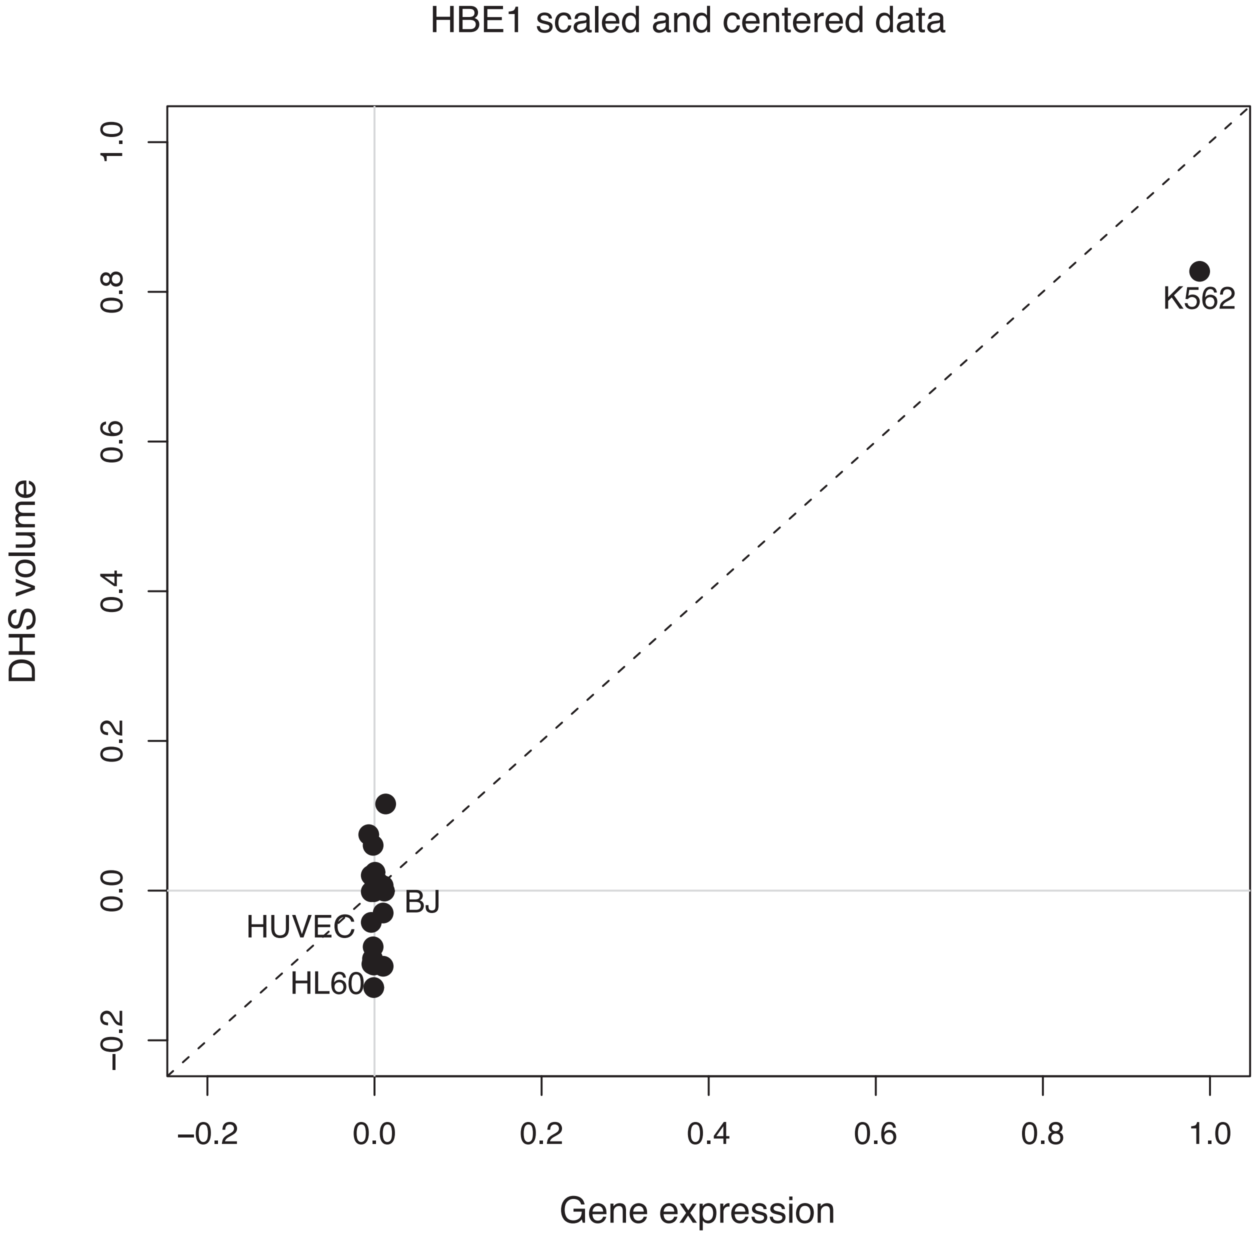


Figure S26: **Scaled and centered gene expression and DHS volume for *HBE1*.** The gene expression and DHS volume [0-1] scaled and medoid centered for all 20 cell-types, across the entire ± 100kb DHS segment. *HBE1* is a clear and singular outlier for K562.

## ARS across all cell-types for HBE1

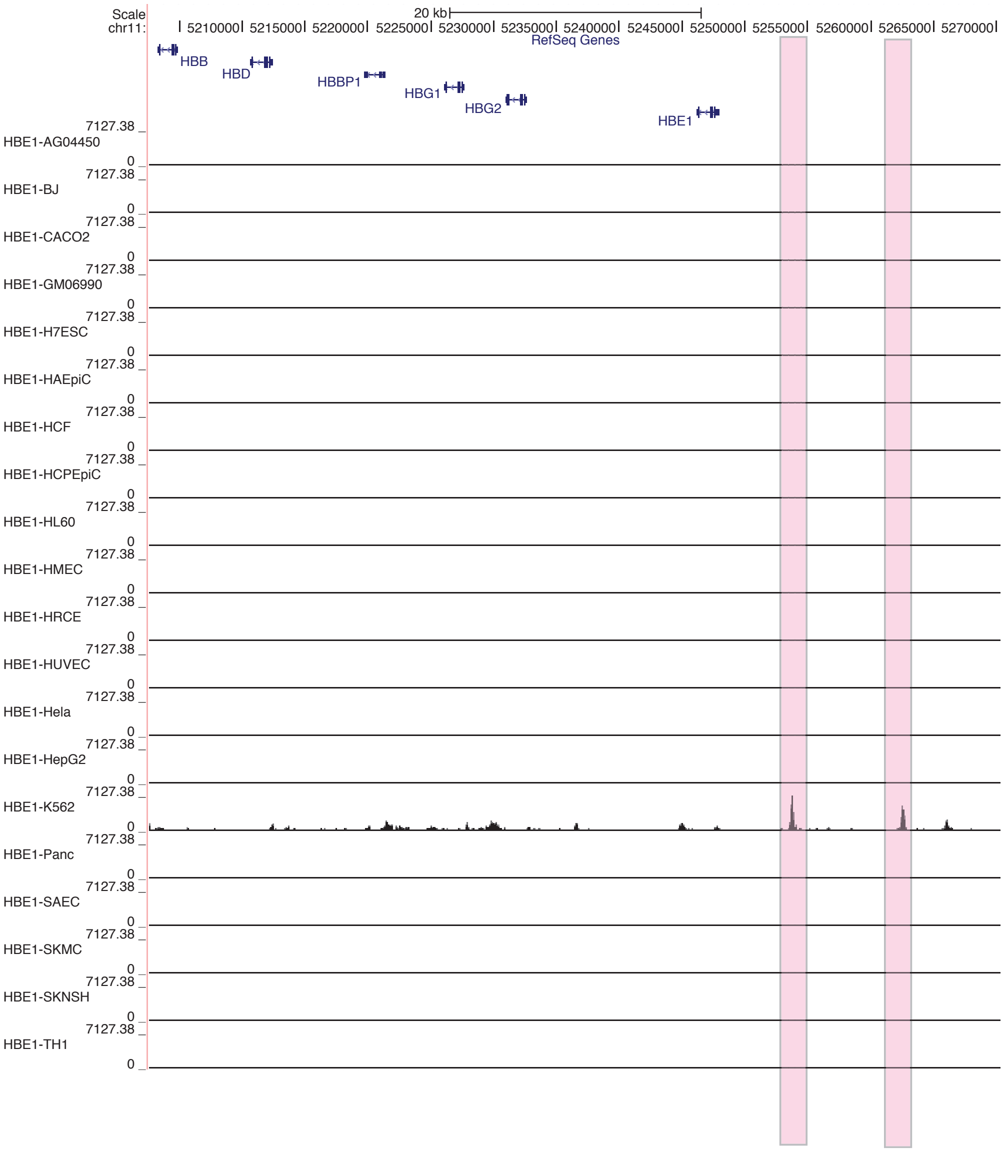


Figure S27: **ARS profiles for *HBE1*.** Local ARS profiles across all 20 cell-types, where the salmon colored bars show that the local ARS profile is markedly different from *HBB*, indicating different regulatory importance of the hypersensitive regions for *HBB* relative to *HBE1*.

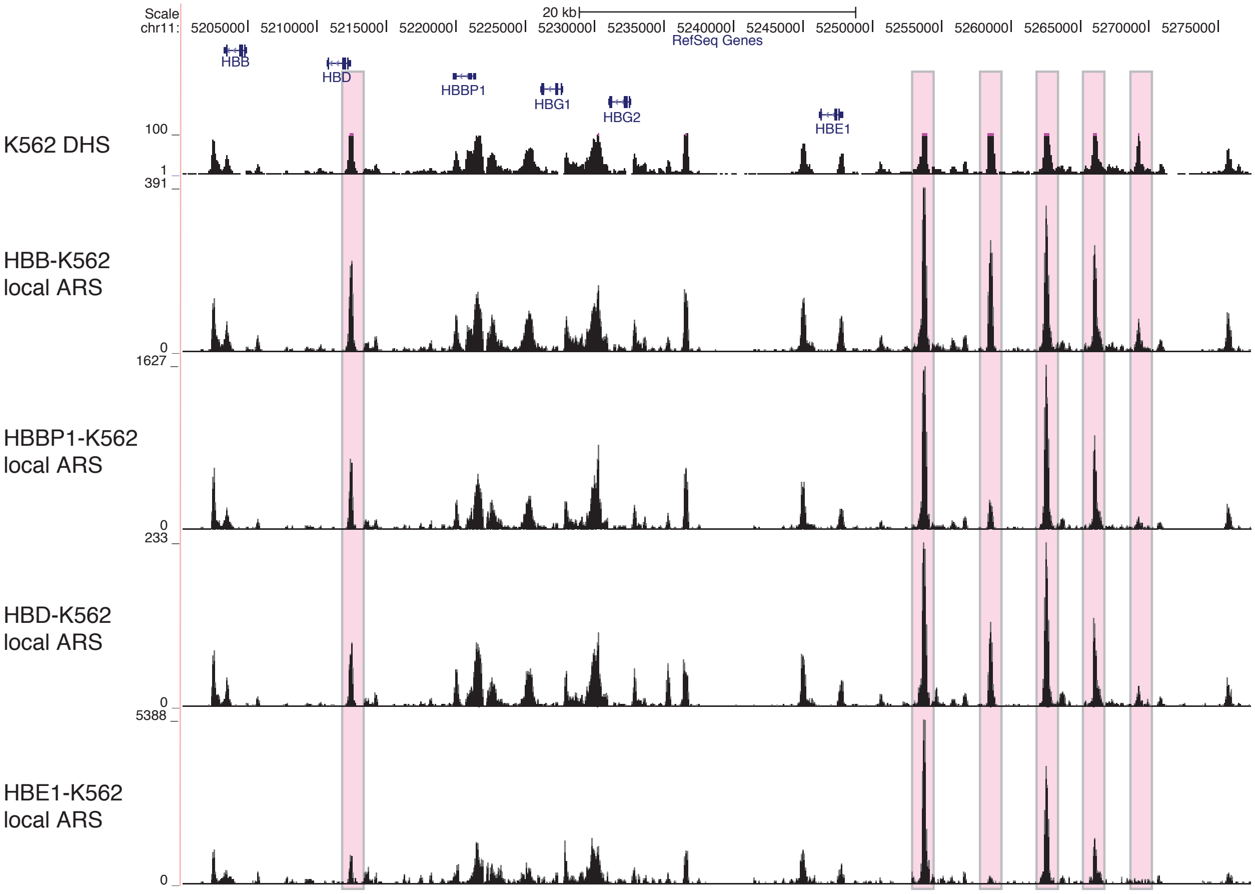


Figure S28: **ARS profiles for entire $\beta$-globin locus.** Local ARS profiles for all genes for which we had expression data in the $\beta$-globin control locus region. The hypersensitive regions are utilized differently by the genes, indicating a difference in regulatory regime. ARS peaks are highlighted by salmon colored bars. The third ARS peak from the left shows significant variation across the genes, despite being chromatin / gene expression concordant in the same cell-type.

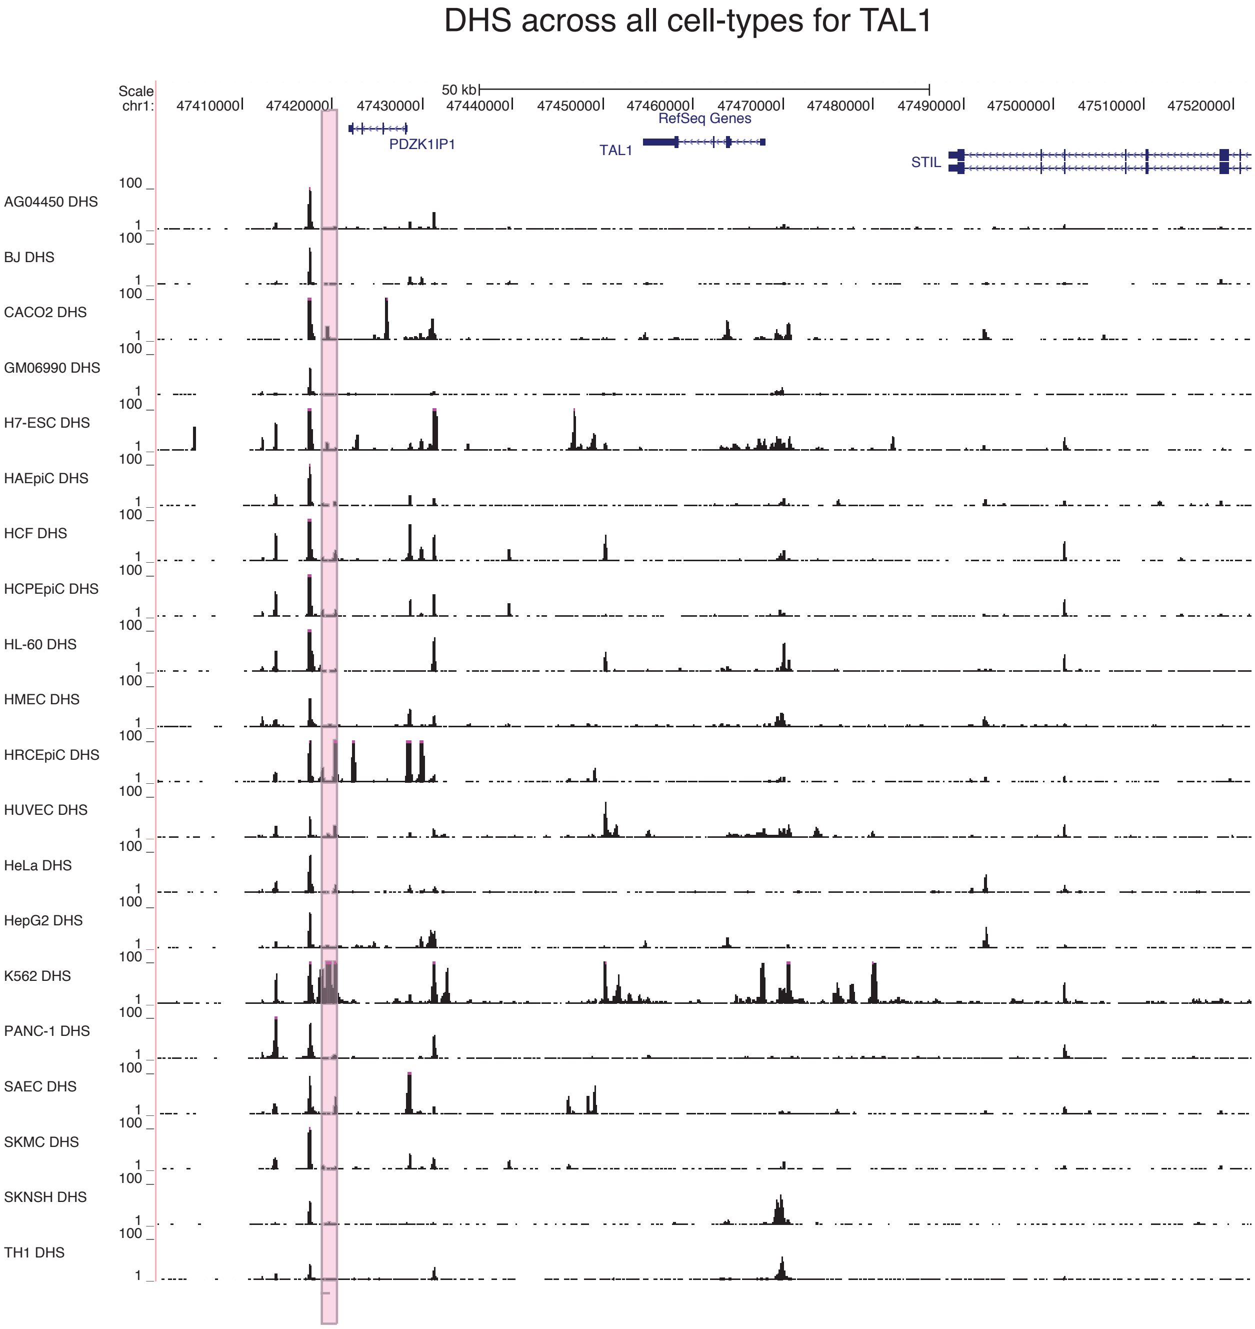


Figure S29: **Raw data DHS fragment counts for *TAL1*.** The DHS values within a region of interest for *TAL1* across all cell-types, where the salmon colored bar indicates the area detected as a local ARS peak for *TAL1*.

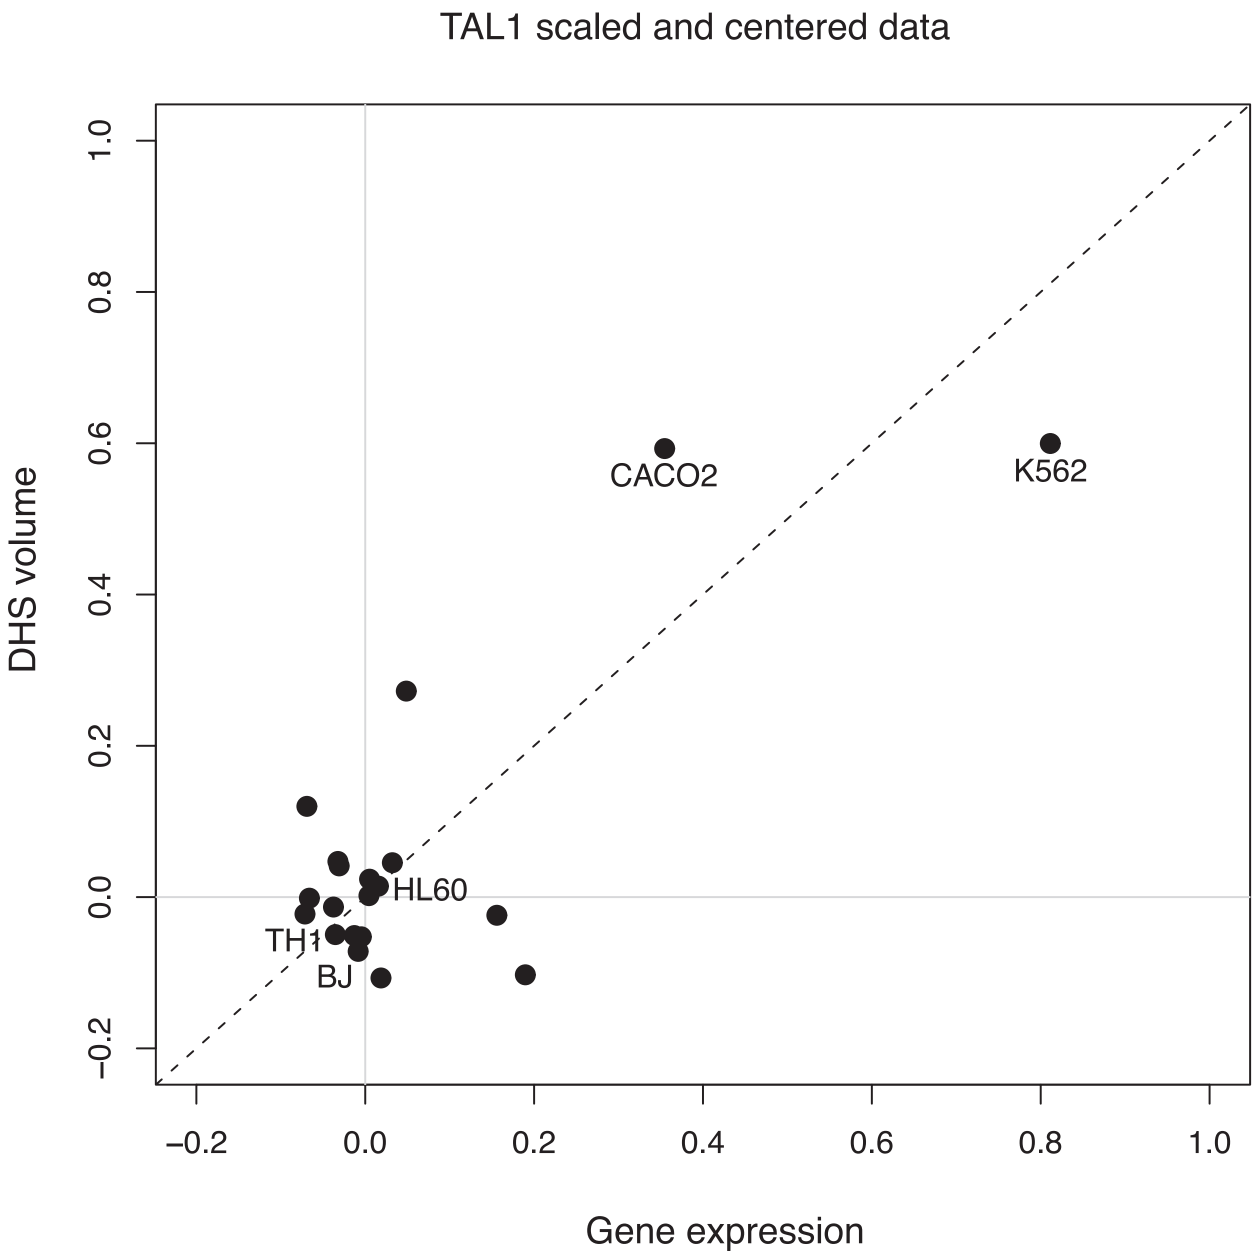


Figure S30: **Scaled and centered gene expression and DHS volume for *TAL1*.** The gene expression and DHS volume [0-1] scaled and medoid centered for all 20 cell-types, across the entire ± 100kb DHS segment. *TAL1* is an outlier for K562, and a secondary outlier for CACO2.

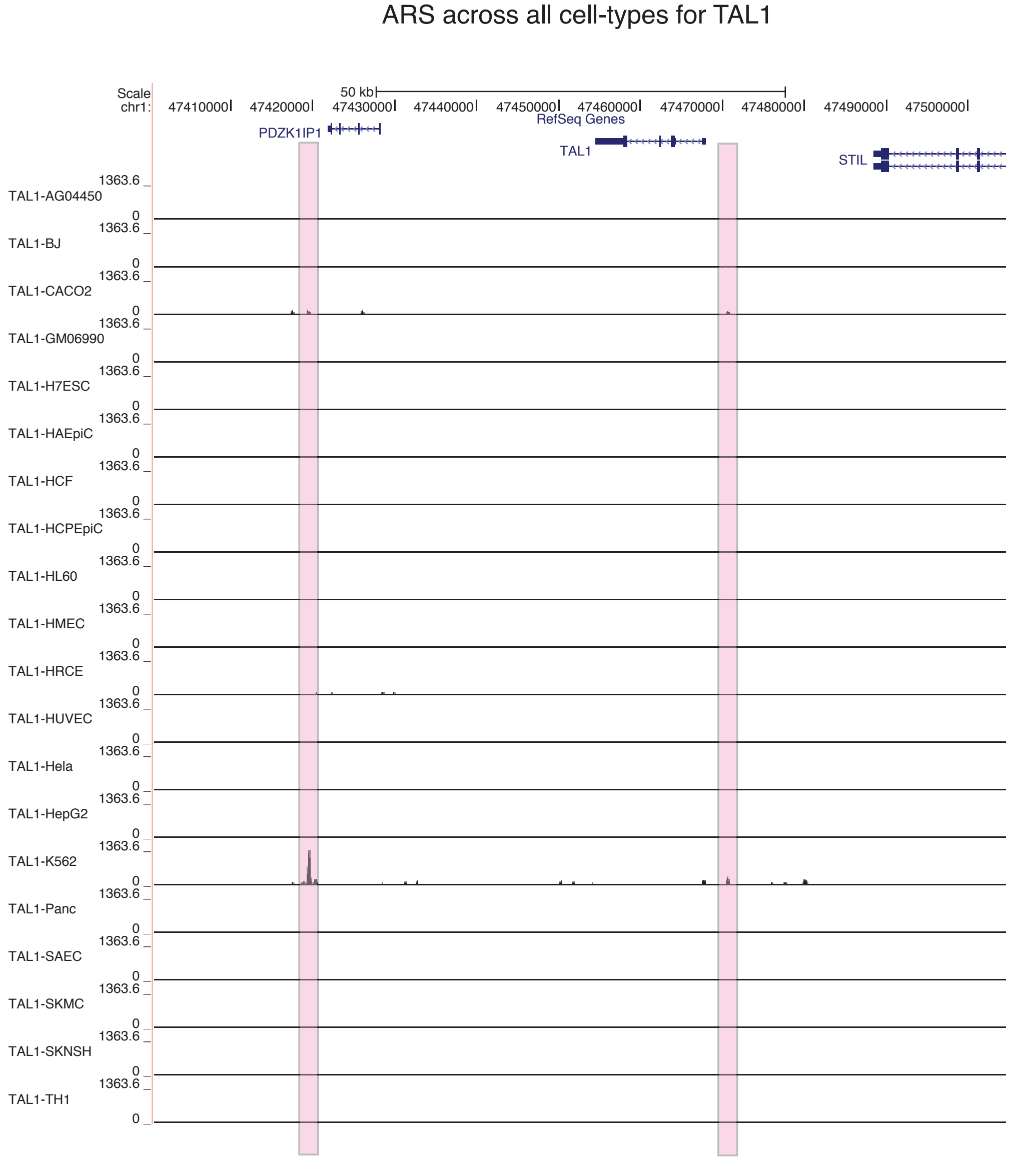


Figure S31: **ARS profiles for *TAL1*.** Local ARS profiles across all 20 cell-types, where the salmon colored bars indicate the ARS peaks. Interestingly, a clear hypersensitive site from Figure S29 does not yield a local ARS peak as it is present in all tissues, and therefore not in cell-type specific concordance with the gene expression values.

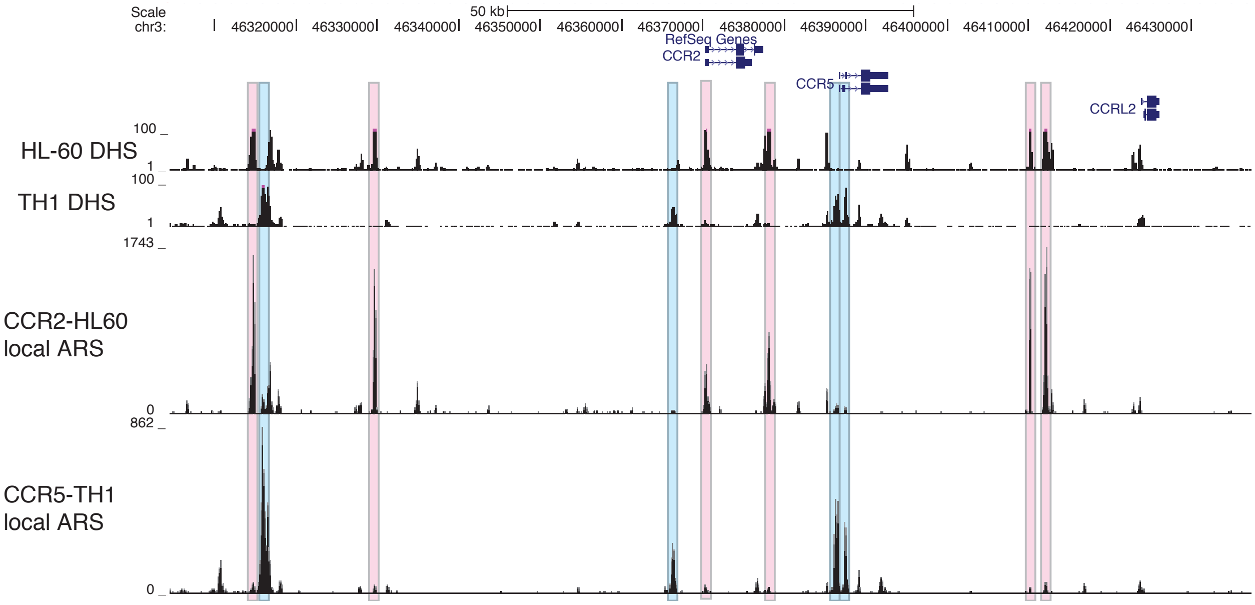


Figure S32: **Distinct local ARS profiles for adjacent genes.** Adjacent significant genes show largely distinct local ARS profiles related to the specific cell-type, indicative of separate regulatory programs. Salmon colored bars show ARS peaks for *CCR2* in HL60 and teal colored bars indicate ARS peaks for *CCR5* in TH1. This example demonstrates the ability of the ARS approach to detect differences in chromatin / gene expression concordance between adjacent genes.

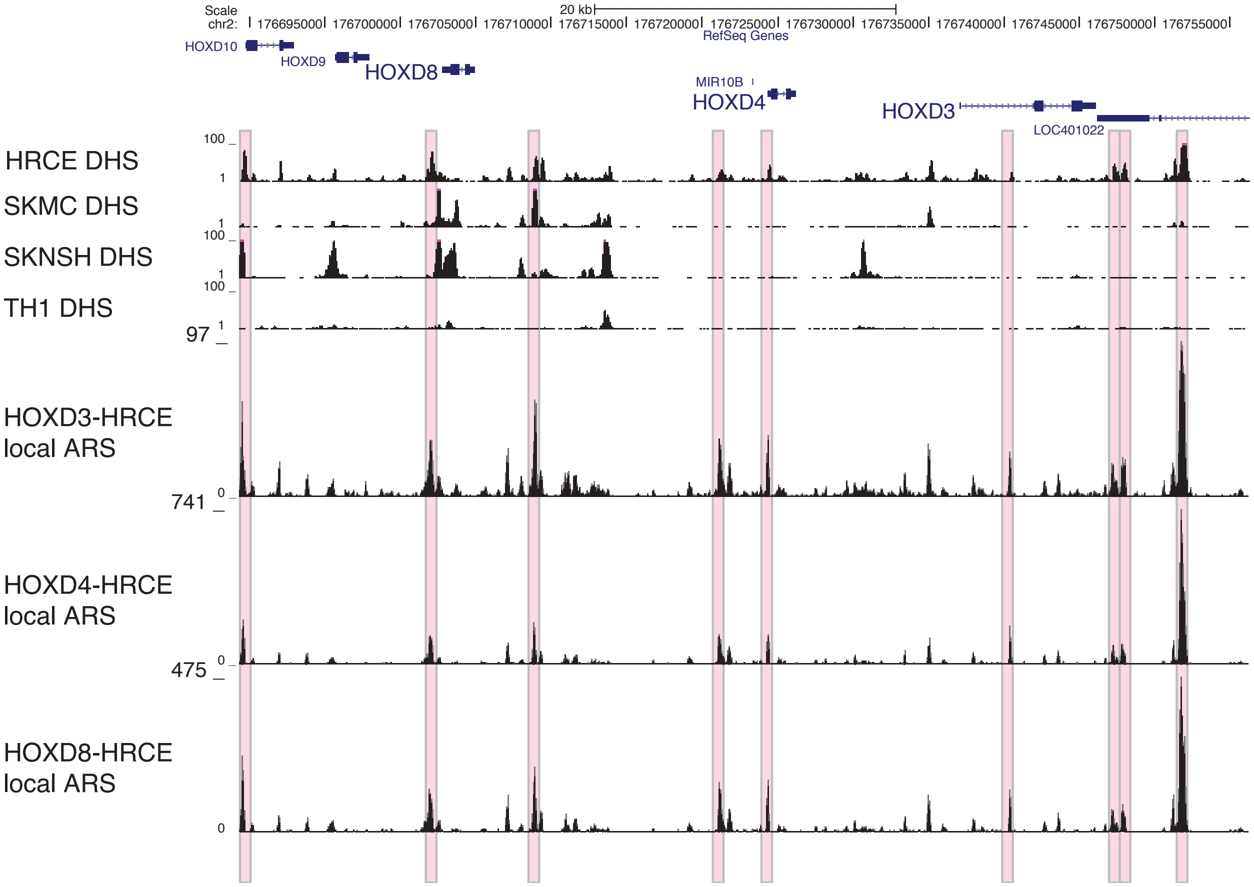


Figure S33: **Shared ARS profile within a single cell-type.** Neighboring *HOXD* genes (*HOXD8, HOXD4, HOXD3*) all significant in HRCE show identical usage of local hypersensitive sites indicative of shared regulatory mechanisms. Salmon colored bars indicate local ARS peaks, which show similar ranking in magnitude within each gene, but differences in total magnitude due to differences in gene expression of the individual genes.

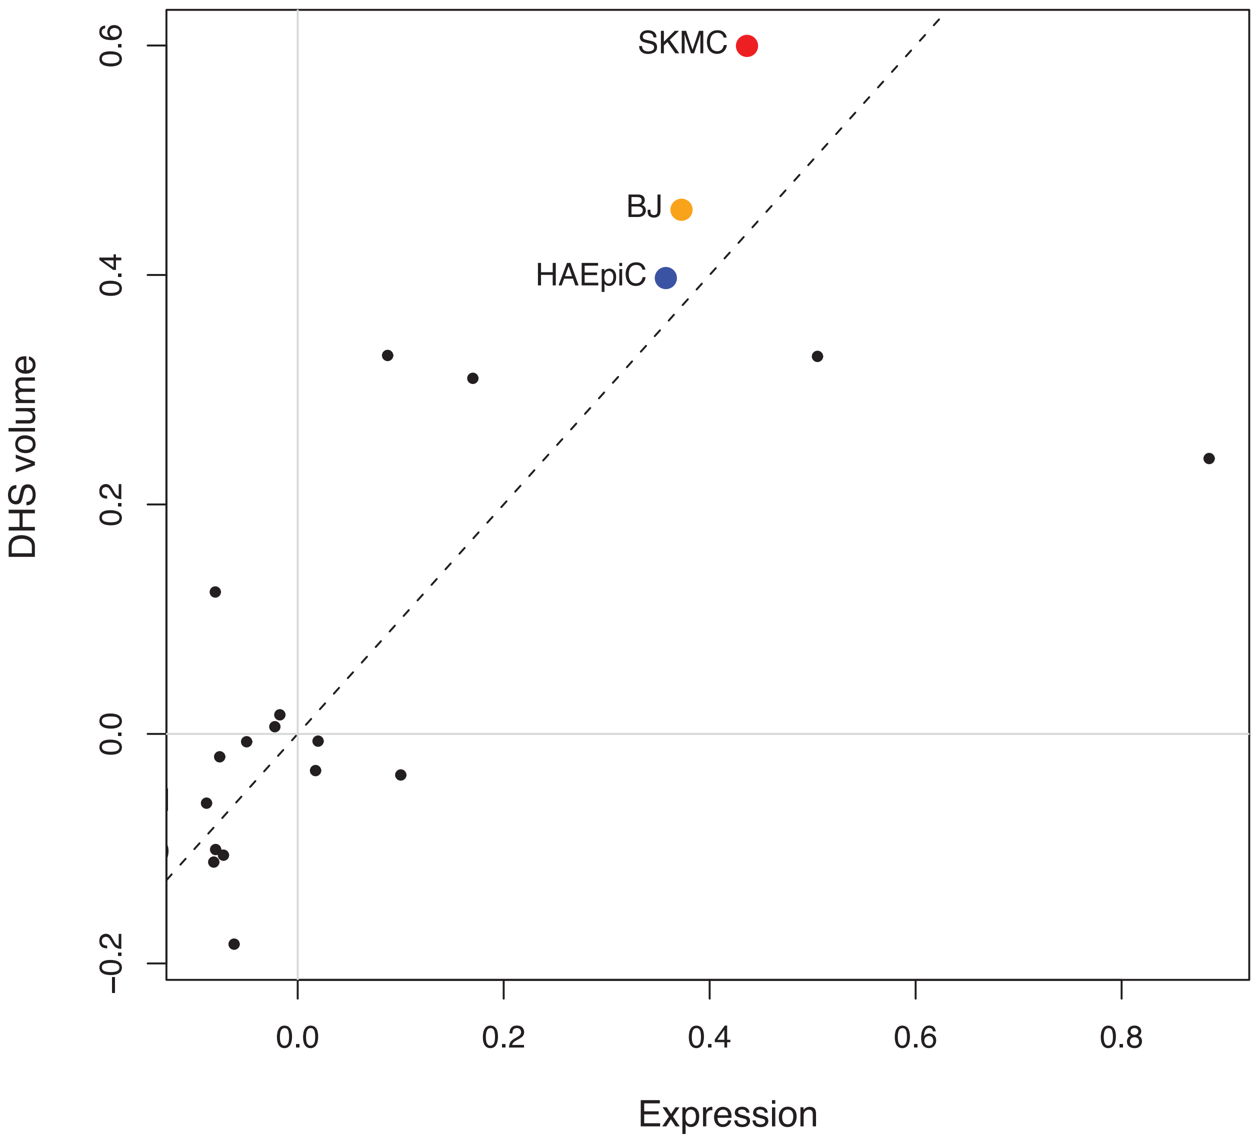


Figure S34: **Sub-maximal outliers for *LOXL2*.** Visualization of the sub-maximal outliers BJ and HAEpiC with similar local ARS profiles as SKMC shown below in Figure S35. While statistical significance is based on $ARS_{max}$, secondary outliers can be seen for other cell-types, indicating shared chromatin / gene expression concordance across cell-types.

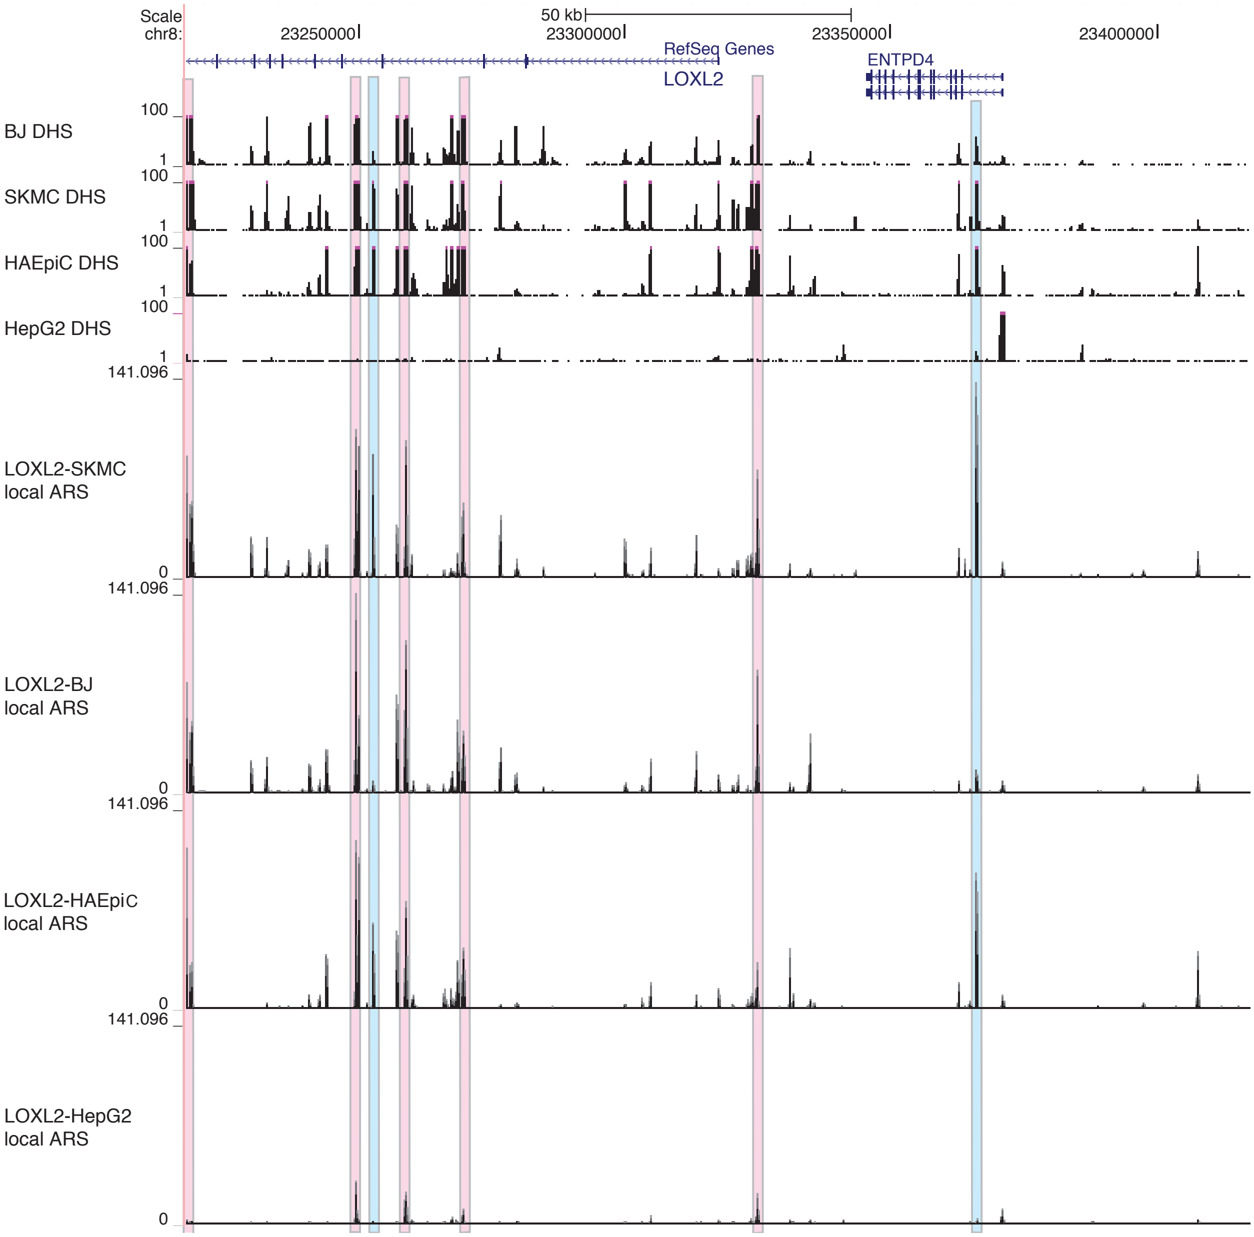


Figure S35: ***LOXL2* share local ARS profiles across cell-types.** While $ARS_{max}$ identified SKMC as the significant outlier, HAEpiC and BJ show large relative local ARS values. Closer inspection shows overlapping utilization of local hypersensitive sites across all three cell-types indicative of possible shared regulatory mechanisms (salmon colored bars). However, individual sites are also detected (teal bars) only shared among SKMC and HAEpiC.
